# Supplementary material for: Online Evasion Attacks on Recurrent Models:The Power of Hallucinating the Future
Source: arXiv:2207.09912 source file (2022-07-08)
Supplement: Supplementary file 2 [file appendix.tex]

\section{Algorithm Details}
\label{appendix:algorithm-detail}
We elaborate on the details of the proposed attack algorithm. Algorithm \autoref{alg:predictive-attack-algorithm-repeated} is the same Algorithm \autoref{alg:predictive-attack-algorithm} in the main paper. It is repeated for readability. This algorithm describes how a current perturbation $\delta_{t}$ is generated.
\begin{algorithm}[h]
\begin{algorithmic}[1]
    \STATE{$ count \gets 0 $} 
    \WHILE{$ count < \text{MAX\_COUNT} $}
        %\STATE{$\hat{x}_{i+1}, ..., \hat{x}_{i+k} \gets Q_{\phi}(x_{1:i}), ..., Q_{\phi}(x_{1:i+k-1})$}\\
        \STATE{$\mathcal{L}_{\text{total}}(\delta_t) \gets \mathcal{L}_{\text{adv}}(x_{t},y^{a}_{t},\delta_{t},h^{\delta}_{t})\newline
        \textcolor{white}{.}\;\;\;\;\;\;\;+ \sum^{t+K}_{i=t+1}\text{E}_{Q_{\phi}(x_i|x_{:i-1})}[\mathcal{L}_{\text{adv}}(x_{i},y^{a}_{i},\delta_{i},h^{\delta}_{i})]$\newline
        \textcolor{white}{.}\;\;\;\;\;\;\;\; using Monte-Carlo to compute $E_{Q_{\phi}}[\cdot]$.}
        \STATE{$\forall i \in [t, t+K],$}
        \STATE{$\delta_i \xleftarrow{} \Pi_{\|{\delta_i}\|_p \leq \epsilon}[\delta_{i} - \alpha \text{sign}(\nabla_{\delta_i}\mathcal{L}_{\text{total}}(\delta_t)]$}
        \STATE{$\delta_i \xleftarrow{} \text{clip}(x_{i}+\delta_i) - x_{i}$}\newline
        \textcolor{white}{.}\;\;\;\;\;\;\;\;\text{It forces a valid range of perturbed inputs.}
        \STATE{$count \xleftarrow{} count + 1$}
    \ENDWHILE
    \RETURN{$\delta_{t}$}
\end{algorithmic}
  \caption{Predictive Attack at time $t$ (Repeated for explanation).}
    \label{alg:predictive-attack-algorithm-repeated}
\end{algorithm}
\\
\textbf{Line 1, 2, 7:} $\delta_{t}$ is computed for $\rm{MAX\_COUNT}$ iterations, and $count$ is an iteration counter. \\
\textbf{Line 3:} Total adversarial loss is computed.
To that end, we predict future inputs ($x_{i}, \forall i \in [t+1, t+K]$) based on the past and predicted observations $x_{:i-1}$ with a predictive model $Q_\phi$. Furthermore, if we use a stochastic predictive model, we can use a mean of adversarial losses computed from multiple predictions (Monte-Carlo). The initial perturbations ($\delta_i, \forall i \in [t+1, t+K]$) are zero vectors. \\
\textbf{Line 4, 5:} For each $i$, we update $\delta_i$ based on Projected Gradient Descent. $\Pi$ restricts the p-norm of $\delta_i$ to be less than $\epsilon$.
\\
\textbf{Line 6:} In addition, $\delta_i$ is needed to be in a valid input range. For instance, a range of pixels of image inputs is [0, 1] or [0, 255].

\section{Model Parameters}
\label{appendix-model-parameters}
\begin{figure*}[t]
\centering
\includegraphics[width=0.80\linewidth]{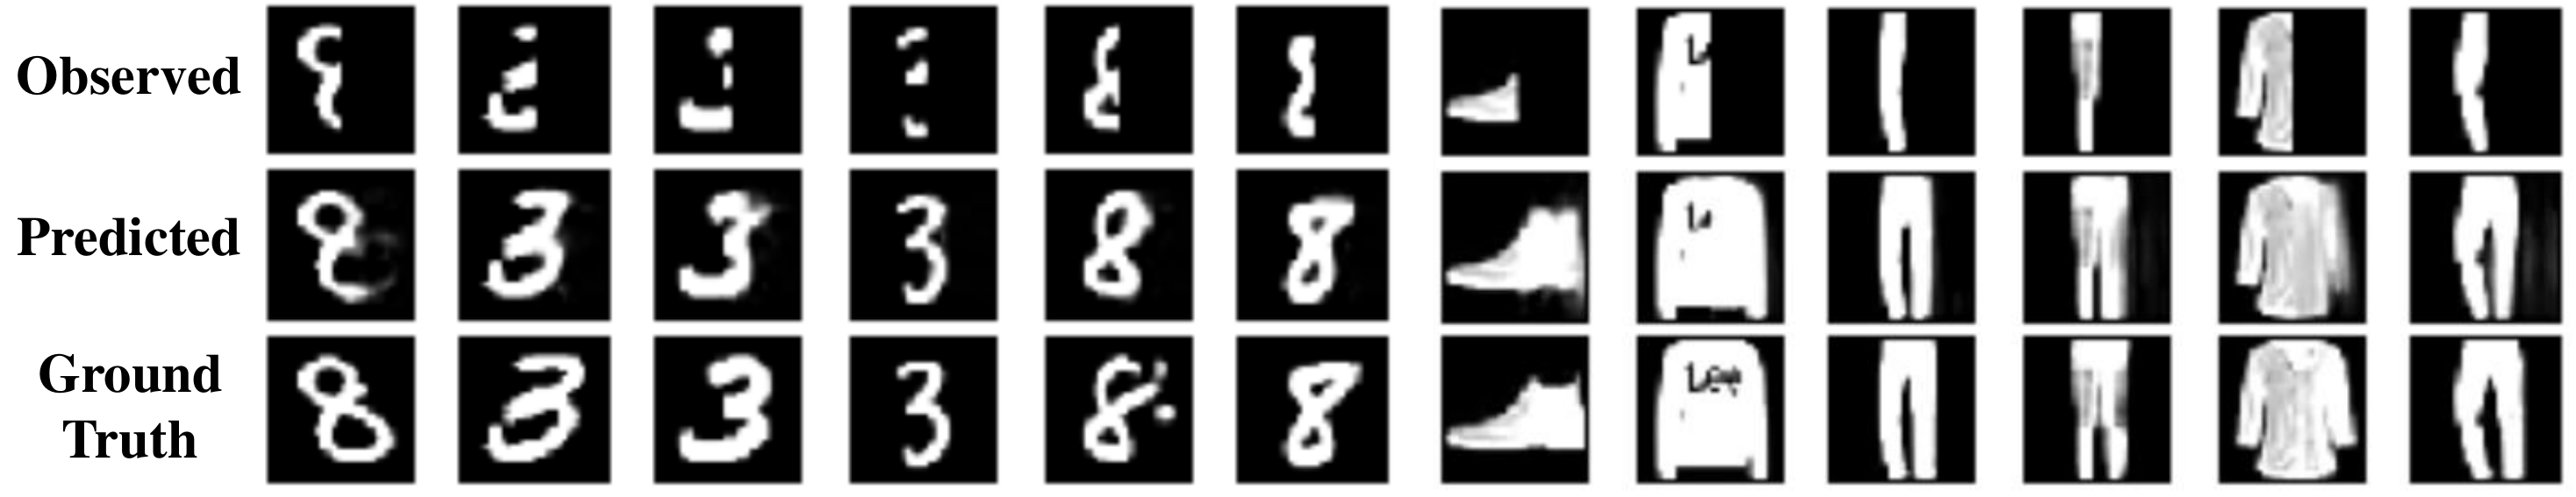}
  \caption{Prediction performance of $Q_\phi$ on MNIST and FashionMNIST.}
  \label{fig:prediction_performance_mnists}
\end{figure*}
We provide detailed information about the parameters for models $(f_\theta, g_\theta)$ and $Q_\phi$. The model structure is shared for MNIST, FashionMNIST, and Mortality, while Udacity uses a different model for high dimensional inputs.
\subsection{MNIST}
{\bf Victim RNN } ($f_\theta$, $g_\theta$)
\begin{itemize}
    \item Input: $x_t \in \mathbb{R}^{28}, h_t \in \mathbb{R}^4$.
    \item Output: $\hat{y}_t \in \mathbb{R}^2$.
\end{itemize}
\begin{enumerate}
    \item LSTM (in=28, hidden=4)
    \item Linear (in=8, out=10, bias=True)
    \item ReLU
    \item Linear (in=10, out=2, bias=True)
\end{enumerate}
{\bf Predictor RNN $Q_\phi$ }% ($f_\theta$, $g_\theta$)
\begin{itemize}
    \item Input: $x_t \in \mathbb{R}^{28}, h_t \in \mathbb{R}^{128}$.
    \item Output: $\hat{x}_{t+1} \in \mathbb{R}^{28}$.
\end{itemize}
\begin{enumerate}
    \item LSTM (in=28, hidden=128)
    \item Linear (in=128, out=150, bias=True)
    \item Dropout (drop\_probability=0.3)
    \item ReLU
    \item Linear (in=150, out=28, bias=True)
\end{enumerate}

\subsection{FashionMNIST}
{\bf Victim RNN } ($f_\theta$, $g_\theta$)
\begin{itemize}
    \item Input: $x_t \in \mathbb{R}^{28}, h_t \in \mathbb{R}^{8}$.
    \item Output: $\hat{y}_t \in \mathbb{R}^{10}$.
\end{itemize}
\begin{enumerate}
    \item LSTM (in=28, hidden=\textcolor{blue}{8})
    \item Linear (in=8, out=10, bias=True)
    \item ReLU
    \item Linear (in=10, out=\textcolor{blue}{10}, bias=True)
\end{enumerate}
{\bf Predictor RNN $Q_\phi$ } %($f_\theta$, $g_\theta$)
\begin{itemize}
    \item Input: $x_t \in \mathbb{R}^{28}, h_t \in \mathbb{R}^{128}$.
    \item Output: $\hat{x}_{t+1} \in \mathbb{R}^{28}$.
\end{itemize}
\begin{enumerate}
    \item LSTM (in=28, hidden=128)
    \item Linear (in=128, out=150, bias=True)
    \item Dropout (drop\_probability=0.3)
    \item ReLU
    \item Linear (in=150, out=28, bias=True)
\end{enumerate}

\subsection{Mortality}
{\bf Victim RNN } ($f_\theta$, $g_\theta$)
\begin{itemize}
    \item Input: $x_t \in \mathbb{R}^{76}, h_t \in \mathbb{R}^{16}$.
    \item Output: $\hat{y}_t \in \mathbb{R}^{2}$.
\end{itemize}
\begin{enumerate}
    \item LSTM (in=\textcolor{blue}{76}, hidden=16)
    \item Linear (in=\textcolor{blue}{16}, out=10, bias=True)
    \item ReLU
    \item Linear (in=10, out=\textcolor{blue}{2}, bias=True)
\end{enumerate}
{\bf Predictor RNN $Q_\phi$ }% ($f_\theta$, $g_\theta$)
\begin{itemize}
    \item Input: $x_t \in \mathbb{R}^{76}, h_t \in \mathbb{R}^{128}$.
    \item Output: $\hat{x}_{t+1} \in \mathbb{R}^{76}$.
\end{itemize}
\begin{enumerate}
    \item LSTM (in=\textcolor{blue}{76}, hidden=128)
    \item Linear (in=128, out=150, bias=True)
    \item Dropout (drop\_probability=0.3)
    \item ReLU
    \item Linear (in=150, out=\textcolor{blue}{76}, bias=True)
\end{enumerate}

\subsection{User}
{\bf Victim RNN } ($f_\theta$, $g_\theta$)
\begin{itemize}
    \item Input: $x_t \in \mathbb{R}^{3}, h_t \in \mathbb{R}^{256}$.
    \item Output: $\hat{y}_t \in \mathbb{R}^{22}$.
\end{itemize}
\begin{enumerate}
    \item LSTM (in=\textcolor{blue}{3}, hidden=\textcolor{blue}{256})
    \item Linear (in=256, out=200, bias=True)
    \item ReLU
    \item Linear (in=200, out=200, bias=True)
    \item ReLU
    \item Linear (in=200, out=200, bias=True)
    \item ReLU
    \item Linear (in=200, out=\textcolor{blue}{22}, bias=True)
\end{enumerate}
{\bf Predictor RNN $Q_\phi$ }% ($f_\theta$, $g_\theta$)
\begin{itemize}
    \item Input: $x_t \in \mathbb{R}^{3}, h_t \in \mathbb{R}^{128}$.
    \item Output: $\hat{x}_{t+1} \in \mathbb{R}^{3}$.
\end{itemize}
\begin{enumerate}
    \item LSTM (in=\textcolor{blue}{3}, hidden=128)
    \item Linear (in=128, out=150, bias=True)
    \item Dropout (drop\_probability=0.3)
    \item ReLU
    \item Linear (in=150, out=\textcolor{blue}{3}, bias=True)
\end{enumerate}

\subsection{Udacity}
{\bf Victim RNN } ($f_\theta$, $g_\theta$)
\begin{itemize}
    \item Input: $x_t \in \mathbb{R}^{64 \times 3}, h_t \in \mathbb{R}^{256}$.
    \item Output: $\hat{y}_t \in \mathbb{R}$.
\end{itemize}
\begin{enumerate}
    \item Conv. (in-channel=3, out-channel=16, kernel-size=16, stride=1)
    \item ReLU
    \item Conv. (in-channel=16, out-channel=16, kernel-size=16, stride=2)
    \item ReLU
    \item Conv. (in-channel=16, out-channel=2, kernel-size=8, stride=2)
    \item LSTM (in=50, hidden=32)
    \item Linear (in=32, out=50, bias=True)    \item ReLU
    \item Linear (in=50, out=1, bias=True)
\end{enumerate}
{\bf Predictor RNN $Q_\phi$ }% ($f_\theta$, $g_\theta$)
\\
$Q_\phi$ consists of two models: 1) Revertible Encoder, and 2) Frame Predictor.
The Revertible Encoder is a revertible function that maps an input image to a feature vector.
The Frame Predictor is a recurrent model that predicts a feature vector of the next time step, based on the current feature vector and a hidden state.
After that, the Revertible Encoder reverts the predicted feature vector and obtains the predicted next input.
Please refer to the original paper of CrevNet \cite{crevnet} and the public implementation\footnote{\url{https://github.com/gnosisyuw/CrevNet-Traffic4cast.git}} for details.
\begin{itemize}
    \item Input: $x_t \in \mathbb{R}^{64 \times 64 \times 3}, h_t \in \mathbb{R}^{512}$.
    \item Output: $\hat{x}_{t+1} \in \mathbb{R}^{64 \times 64 \times 3}$.
\end{itemize}
\begin{enumerate}
    \item Revertible Encoder (in=$64 \times 64 \times 3$, out=512)
    \item Frame Predictor (in=512, out=512)
\end{enumerate}

\subsection{Energy}
{\bf Victim RNN } ($f_\theta$, $g_\theta$)
\begin{itemize}
    \item Input: $x_t \in \mathbb{R}^{27}, h_t \in \mathbb{R}^{16}$.
    \item Output: $\hat{y}_t \in \mathbb{R}$.
\end{itemize}
\begin{enumerate}
    \item LSTM (in=\textcolor{blue}{27}, hidden=\textcolor{blue}{16})
    \item Linear (in=16, out=200, bias=True)
    \item ReLU
    \item Linear (in=200, out=200, bias=True)
    \item ReLU
    \item Linear (in=200, out=200, bias=True)
    \item ReLU
    \item Linear (in=200, out=\textcolor{blue}{1}, bias=True)
\end{enumerate}
{\bf Predictor RNN $Q_\phi$ }% ($f_\theta$, $g_\theta$)
\begin{itemize}
    \item Input: $x_t \in \mathbb{R}^{27}, h_t \in \mathbb{R}^{128}$.
    \item Output: $\hat{x}_{t+1} \in \mathbb{R}^{27}$.
\end{itemize}
\begin{enumerate}
    \item LSTM (in=\textcolor{blue}{27}, hidden=1024)
    \item Linear (in=1024, out=150, bias=True)
    \item ReLU
    \item Linear (in=150, out=\textcolor{blue}{27}, bias=True)
\end{enumerate}

% \section{Attack Parameters}
% We choose the following attack parameters. Note that the following parameters are enough to use the available perturbation budget $\epsilon$, $\epsilon < \alpha \times \text{MAX\_COUNT}$.\\
% \begin{itemize}
%     \item MAX\_ITERS$=64$
%     \item $\alpha=1.5 \times \epsilon /$MAX\_ITERS
% \end{itemize}

\section{Mathematical Formation of Metrics in Experiments}
We provide mathematical formation of attack performance metric for each type of task.
\paragraph{Classification Tasks.}
We measure Targeted Attack Success Ratio (TASR), a fraction of time steps where predicted labels are matched to target labels ($y^{a}_{i}$) over the number of total time steps ($L$). $\mathbf{1}[\cdot]$ is an indicator function.
\begin{gather*}
\text{TASR} = \frac{\sum^{L}_{i=1}{\textbf{1}[{f_{\theta}(x_i+\delta_{i},h^{\delta}_i)=y^{a}_i}}]}{L}
\end{gather*}
\paragraph{Regression Tasks.} We measure Targeted Mean Squared Error (TMSE) between predicted values and target values.
\begin{gather*}
\text{TSME} = \frac{1}{L}\sum^{L}_{i=1}{(f_{\theta}(x_i+\delta_{i},h^{\delta}_i)-y^{a}_i)^2}
\end{gather*}

\begin{figure}
\centering
\includegraphics[width=1.0\linewidth]{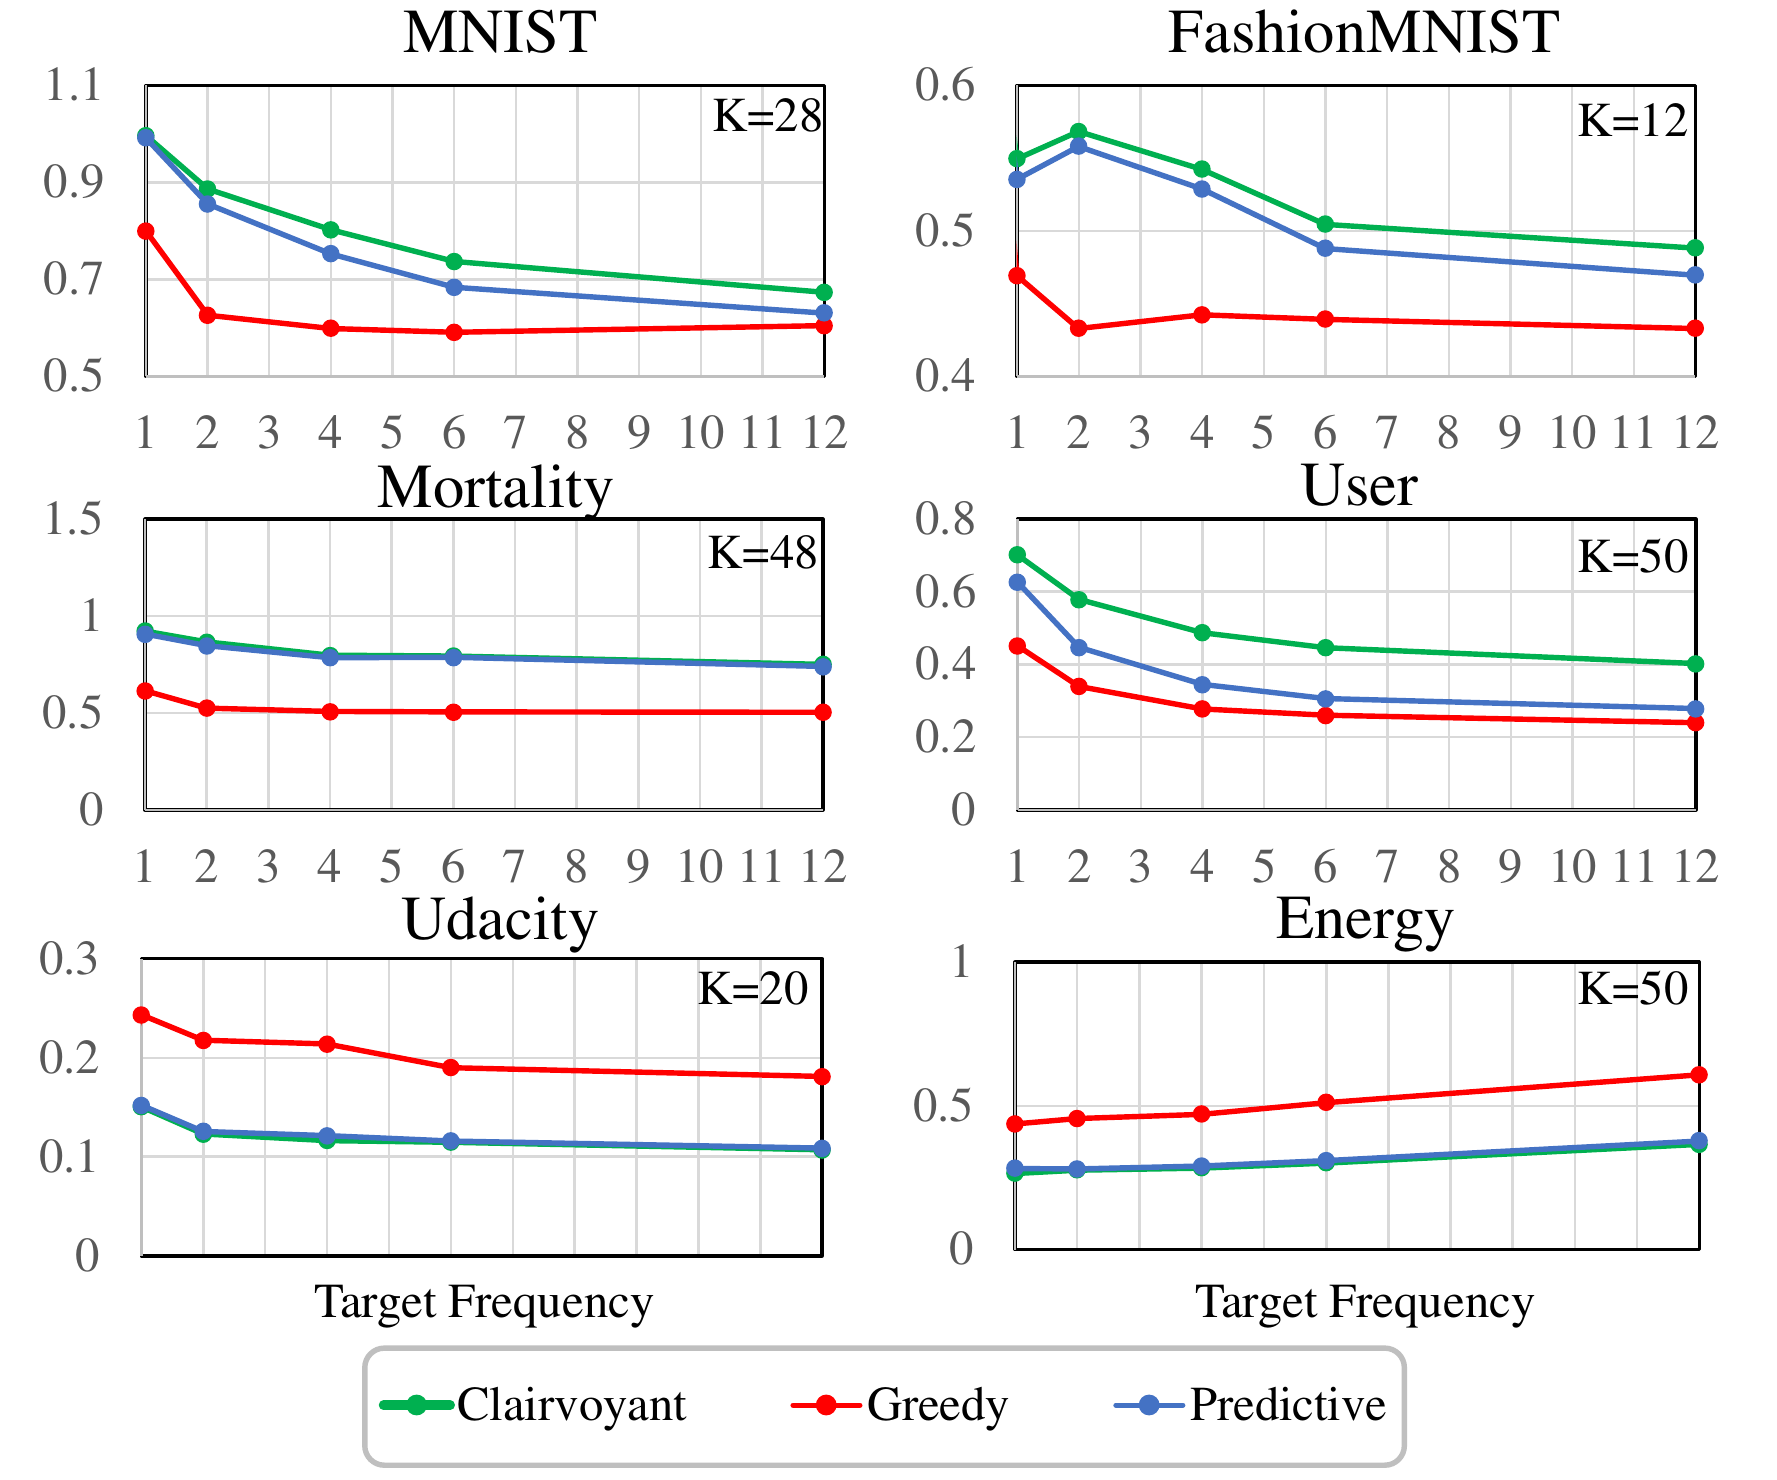}
  \caption{Attack Performances increasing the target frequency. Predictive Attack shows consistent orders of attack performances to \autoref{fig:performance-evaluation-predictive}.}
  \label{fig:multi-wave}
\end{figure}

\section{Prediction Performance}
\label{appendix:prediction-performance}

\begin{figure}
\centering
\includegraphics[width=1.0\linewidth]{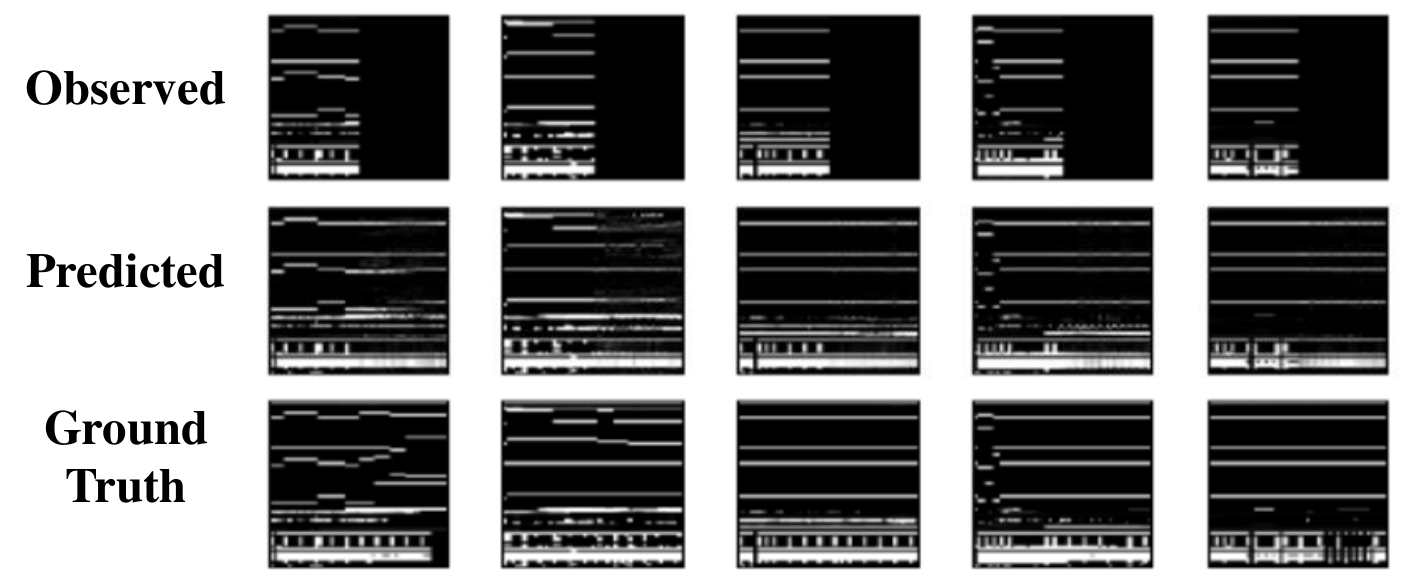}
  \caption{Prediction performance of $Q_\phi$ on Mortality. $76$ dimensions of one-hot encoding and real-valued data, $L=48$.}
  \label{fig:prediction_performance_mortality}
\end{figure}

\begin{figure}
\centering
\includegraphics[width=1.0\linewidth]{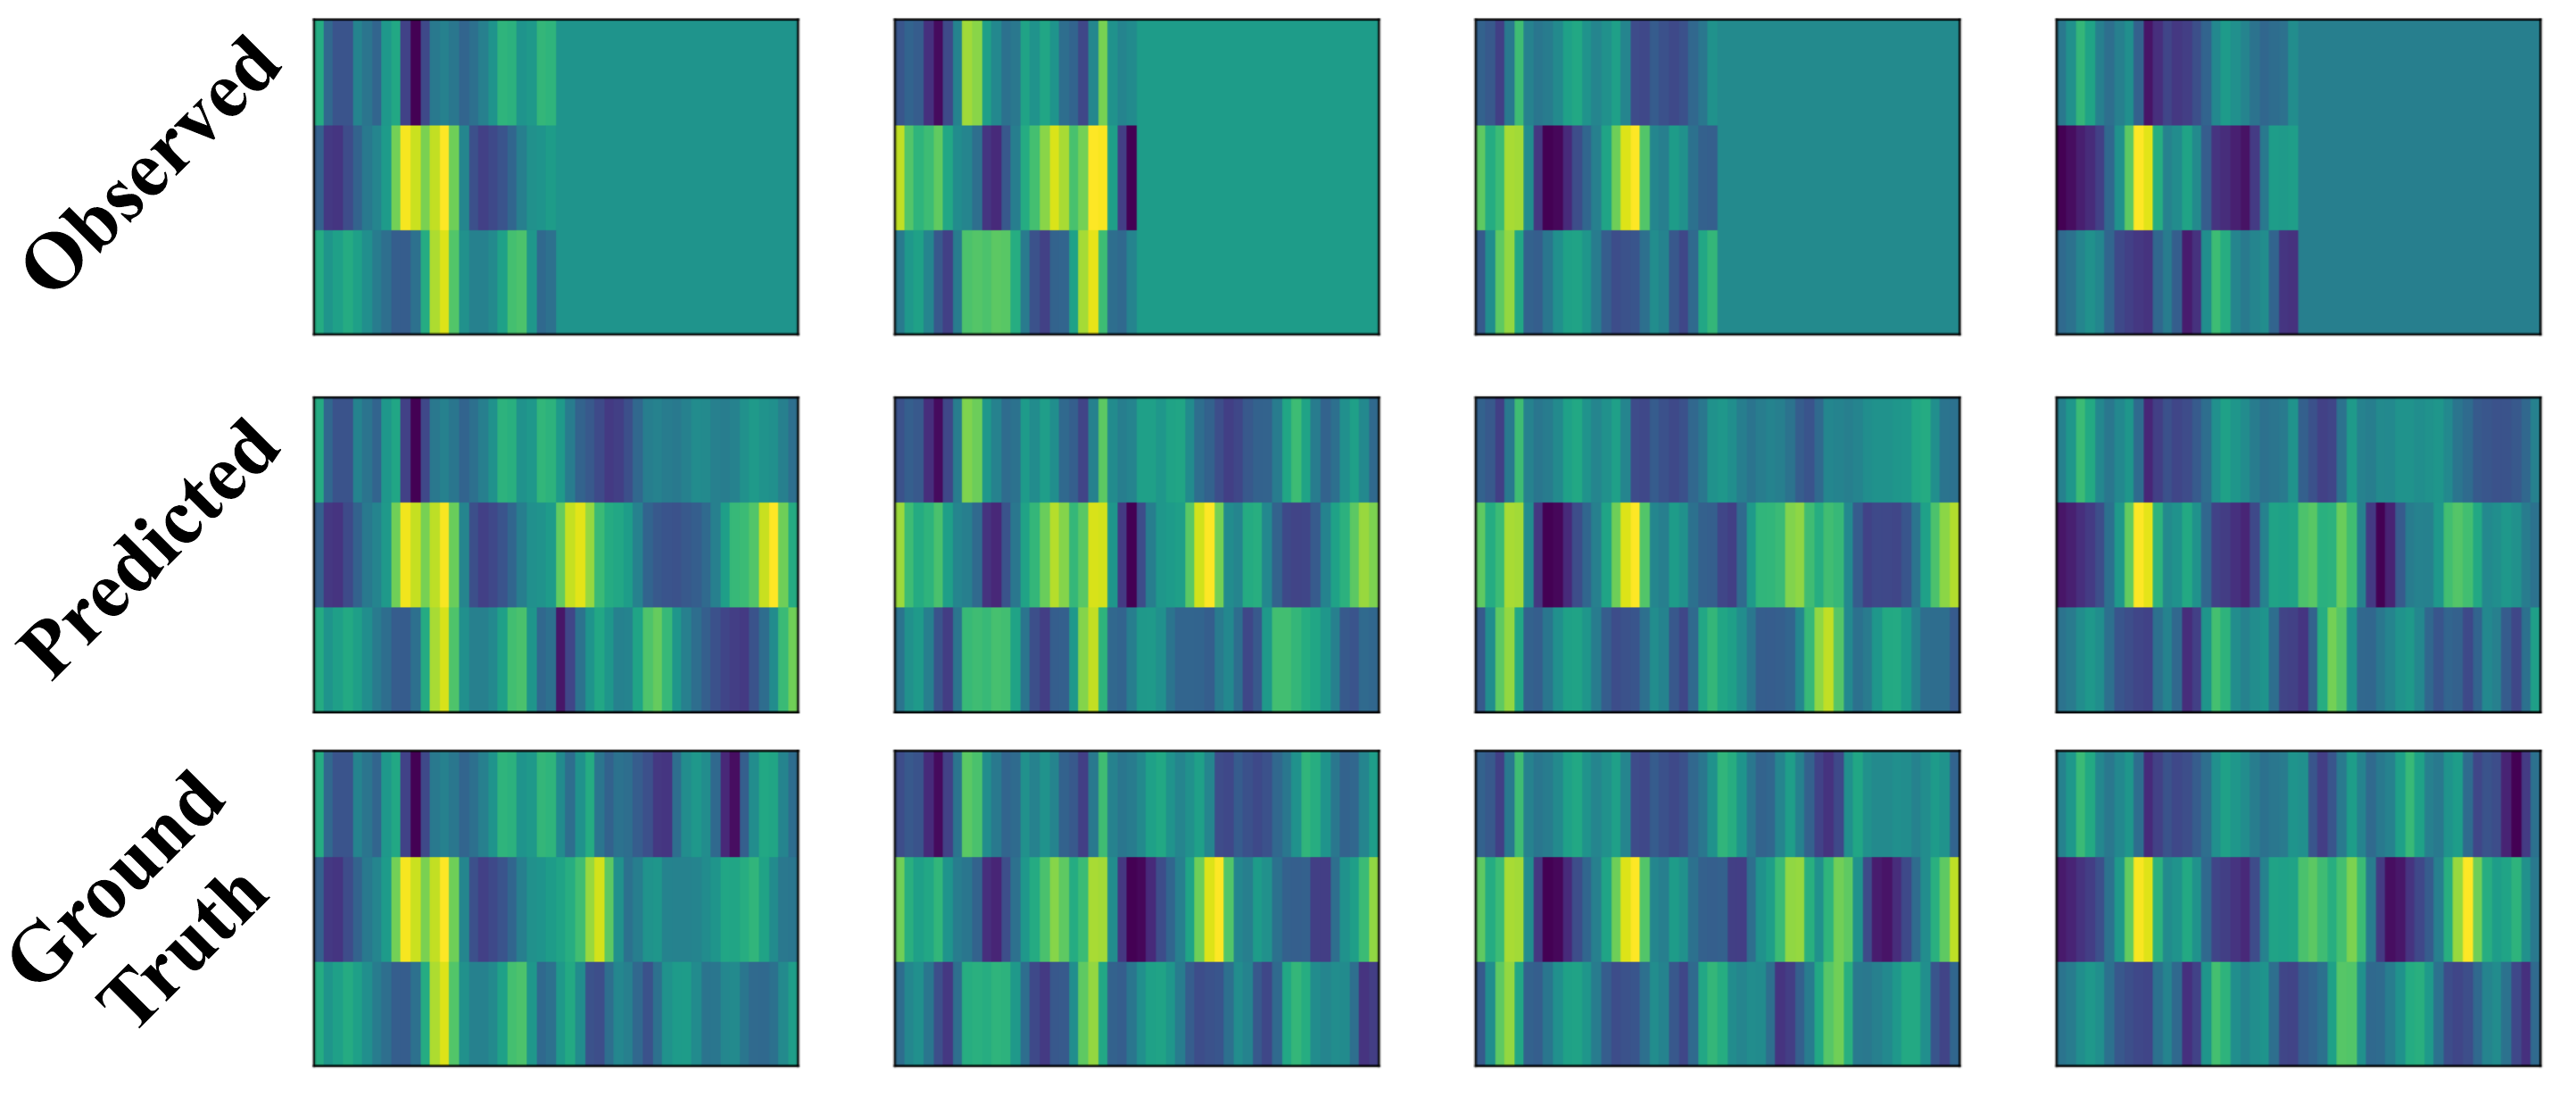}
  \caption{Prediction performance of $Q_\phi$ on User. $3$ dimensions of real values, $L=50$.}
  \label{fig:prediction_performance_user}
\end{figure}

\begin{figure*}
\centering
\includegraphics[width=0.80\linewidth]{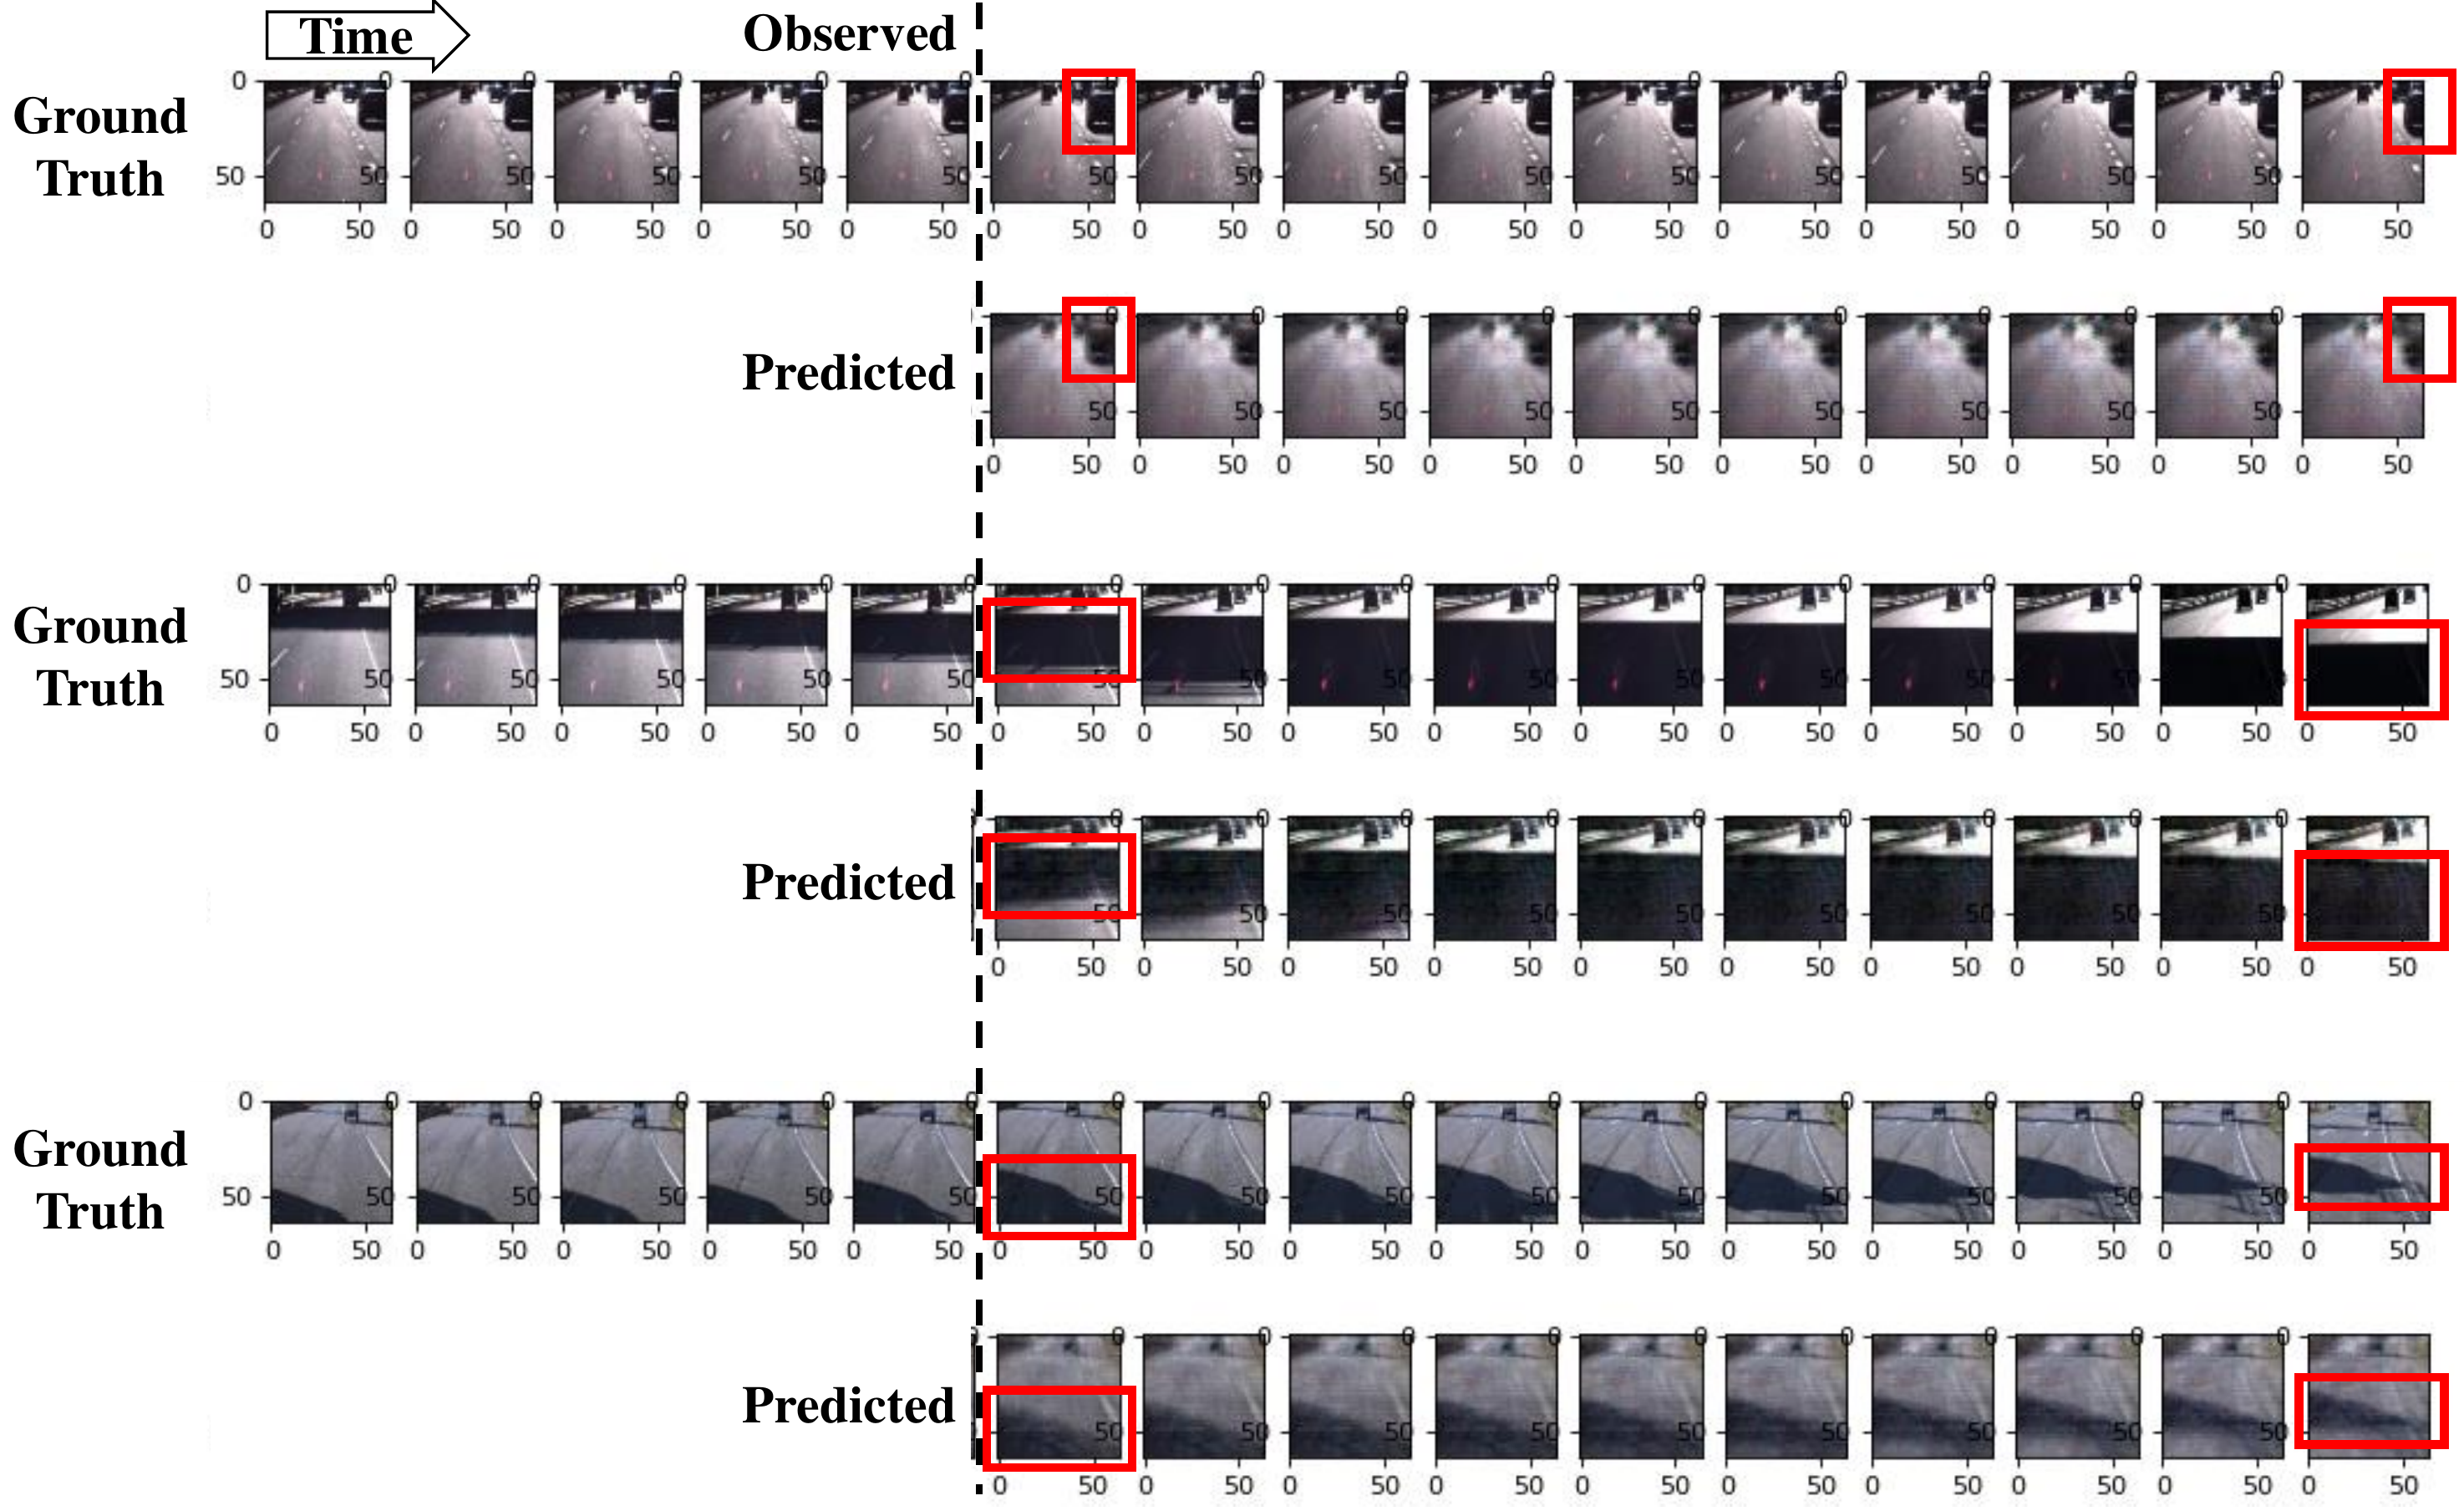}
  \caption{Prediction performance of $Q_\phi$ on Udacity.}
  \label{fig:prediction_performance_udacity}
\end{figure*}

\begin{figure}
\centering
\includegraphics[width=1.0\linewidth]{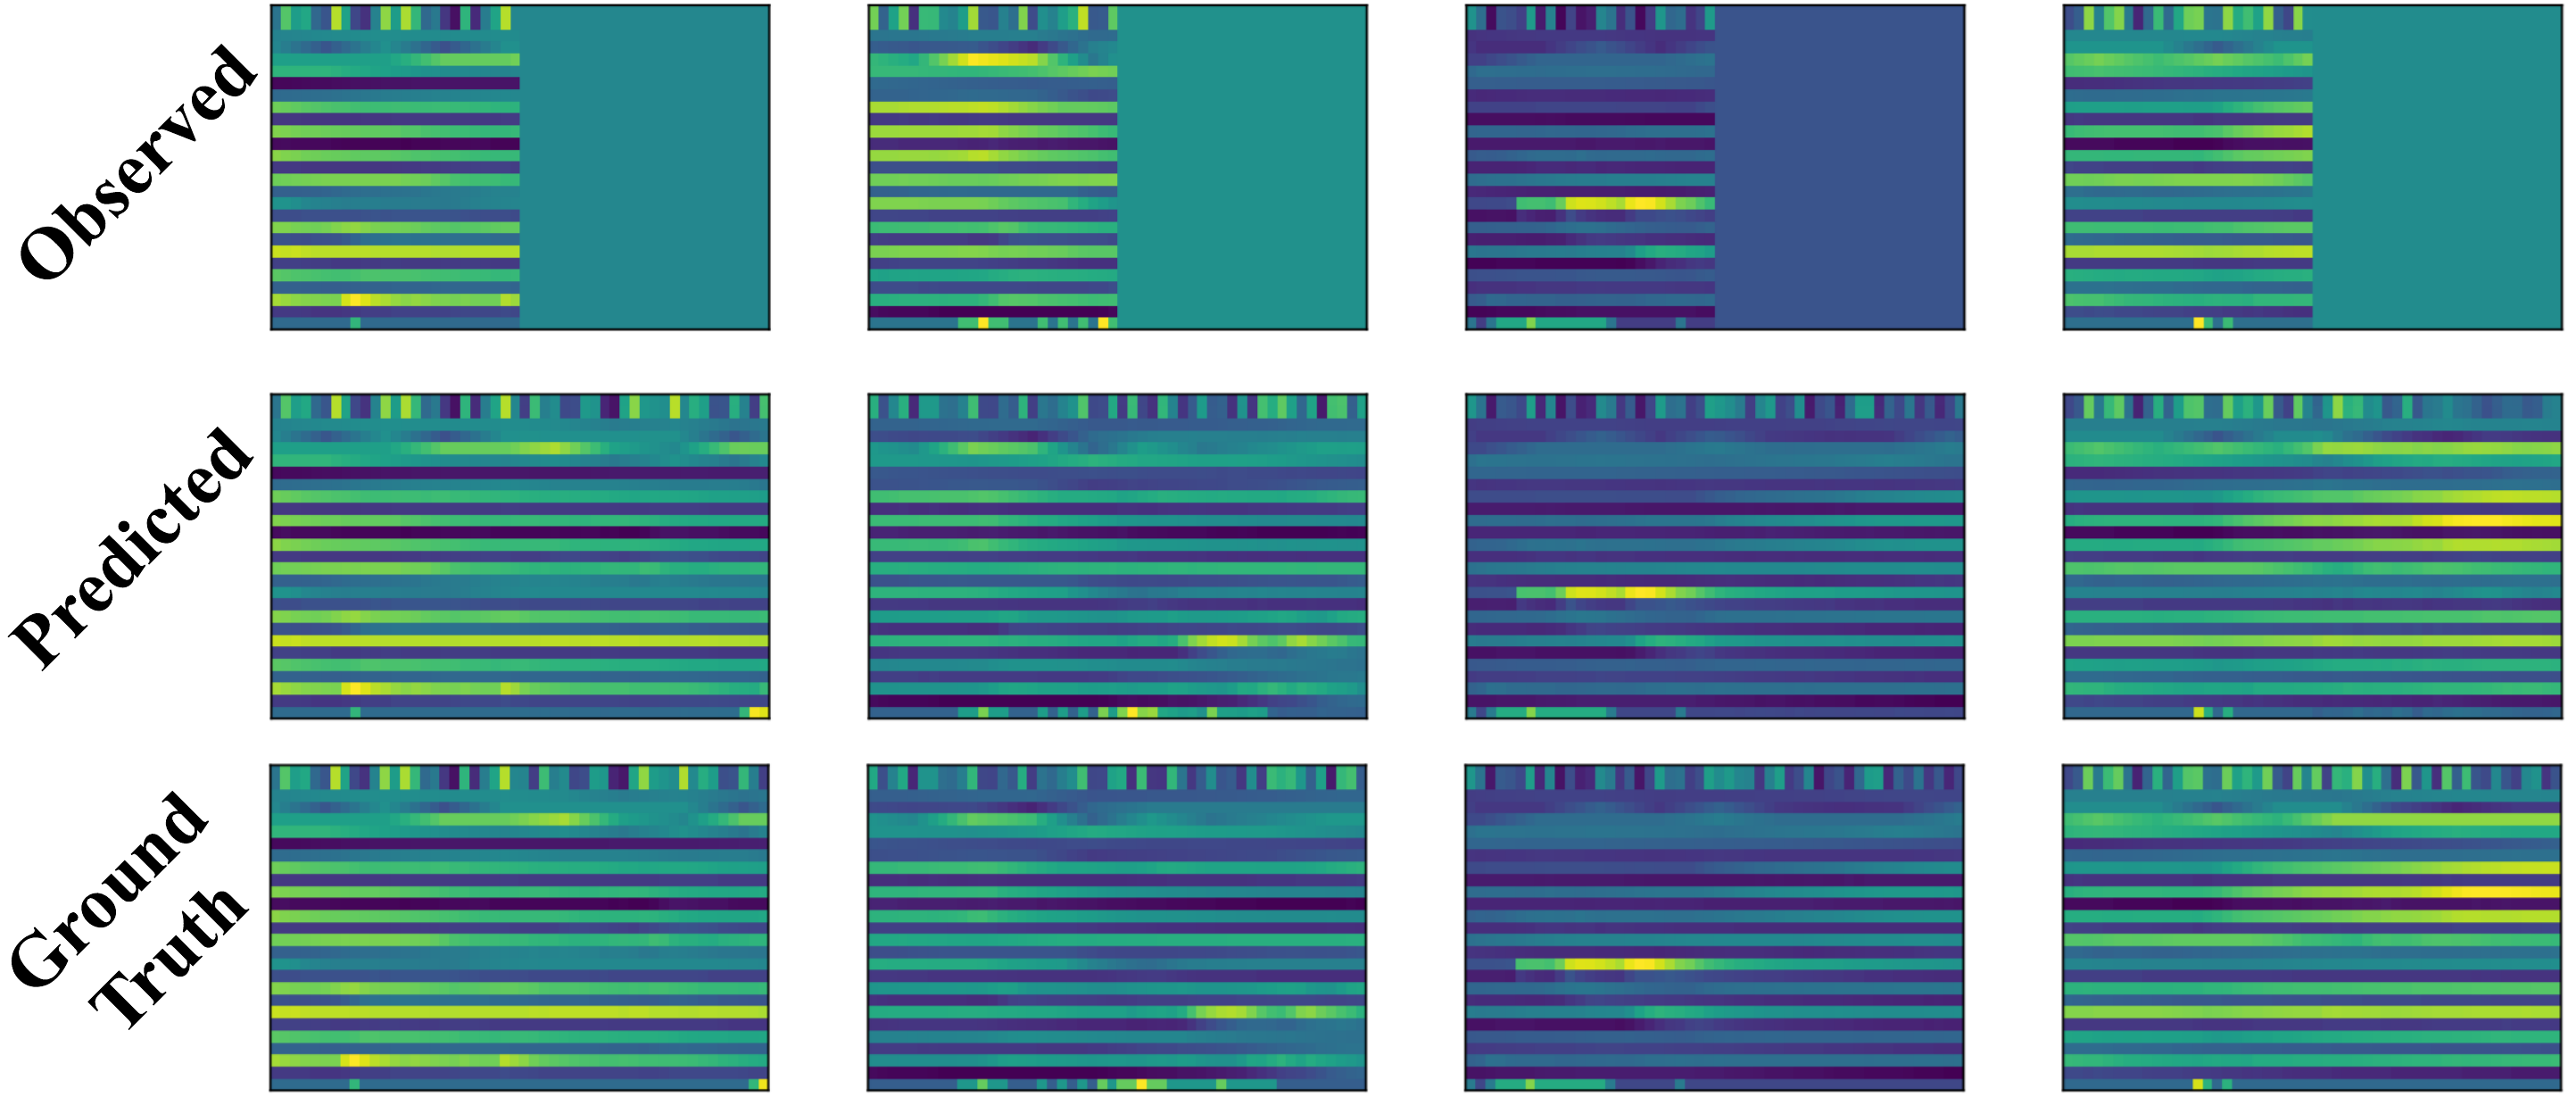}
  \caption{Prediction performance of $Q_\phi$ on Energy. $27$ dimensions of real values, $L=50$.}
  \label{fig:prediction_performance_energy}
\end{figure}
%\BG{explain figure 10: real valued, one hot encoding 48 $\times $76}
To demonstrate the performance of $Q_\phi$, which is important for the Predictive Attack, we present the prediction results in Figure \ref{fig:prediction_performance_mnists}, \ref{fig:prediction_performance_mortality},
\ref{fig:prediction_performance_user},
\ref{fig:prediction_performance_udacity}, and \ref{fig:prediction_performance_energy}.
Given a partial early observations of a sequence $\boldsymbol{x}$, $Q_\phi$ predicts the rest of the sequence. For MNIST, FashionMNIST, and Mortality, we restrict the observation to the first half ($L/2$). We find $Q_\phi$ performs well on the datasets.
Especially, $Q_\phi$ finds a natural extension of observed strokes of a digit. $Q_\phi$  also seems to learn the symmetric property of clothing.
$Q_\phi$  finds the characteristics of Mortality: the composition of one-hot encoding (top-part) and real-valued (bottom-part) data. It produces realistic data, although some one-hot encoding is not correct due to its randomness.

For Udacity, $Q_\phi$ observes the first five frames of road scenes and predicts the rest.  We can see that  $Q_\phi$ captures the dynamics of near vehicles and shadows.

\section{Adversarial Examples}
\label{appendix:adversarial-examples}
To demonstrate the imperceptibility of perturbations, we present adversarial examples generated by Predictive Attack in Figure \ref{fig:adversarial_examples_mnists}, \ref{fig:adversarial_examples_mortality},
\ref{fig:adversarial_examples_user}, \ref{fig:adversarial_examples_udacity}, and
\ref{fig:adversarial_examples_energy}. We verify that the perturbations are hard to notice, although they fool the victim RNNs, achieving 0.83, 0.80, 0.38 and 1.16 evaluation metric, respectively for MNIST, FashionMNIST, Mortality, and Udacity.
\begin{figure*}[t]
\centering
\includegraphics[width=0.80\linewidth]{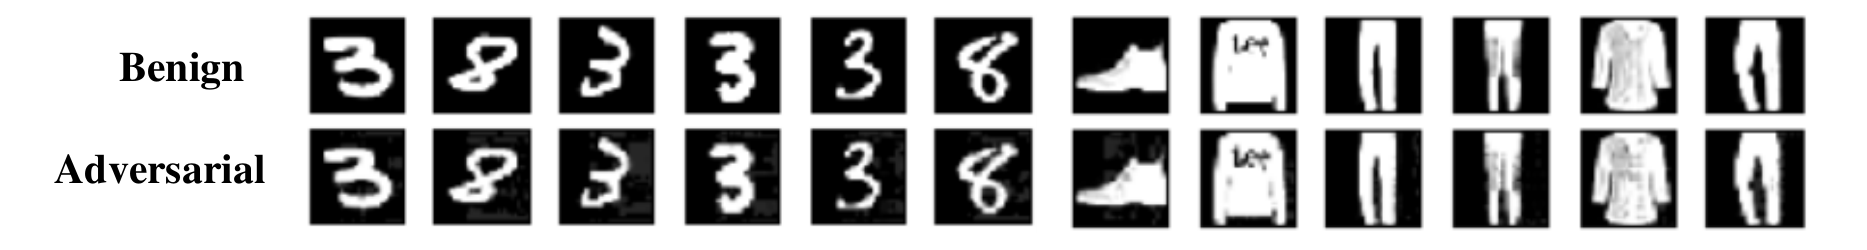}
  \caption{Adversarial examples of Predictive Attack on MNIST and FashionMNIST.
  $\ell_\infty \; \epsilon = 0.15.$}
  \label{fig:adversarial_examples_mnists}
\end{figure*}

\begin{figure}
\centering
\includegraphics[width=1.0\linewidth]{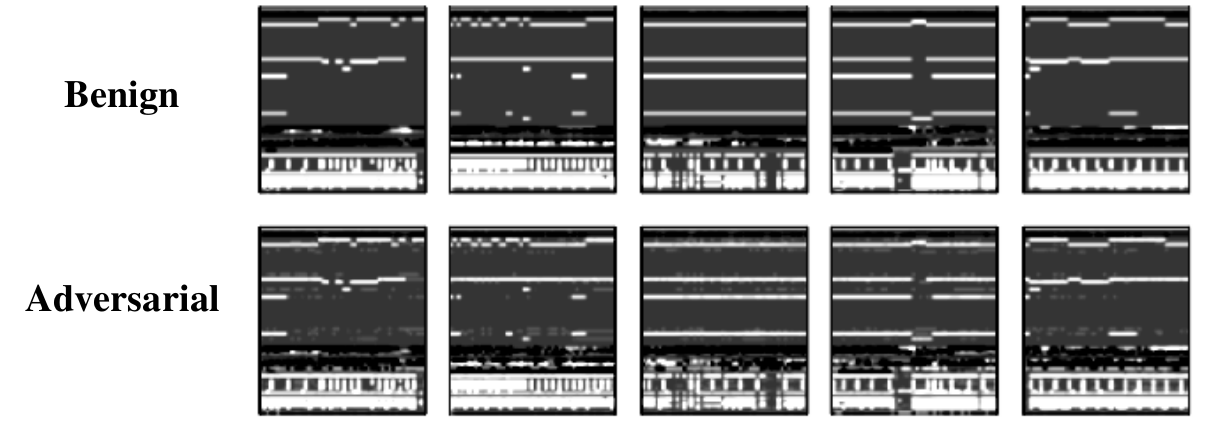}
  \caption{Adversarial examples of Predictive Attack on Mortality. $\ell_\infty \; \epsilon = 0.15.$}
  \label{fig:adversarial_examples_mortality}
\end{figure}

\begin{figure}
\centering
\includegraphics[width=1.0\linewidth]{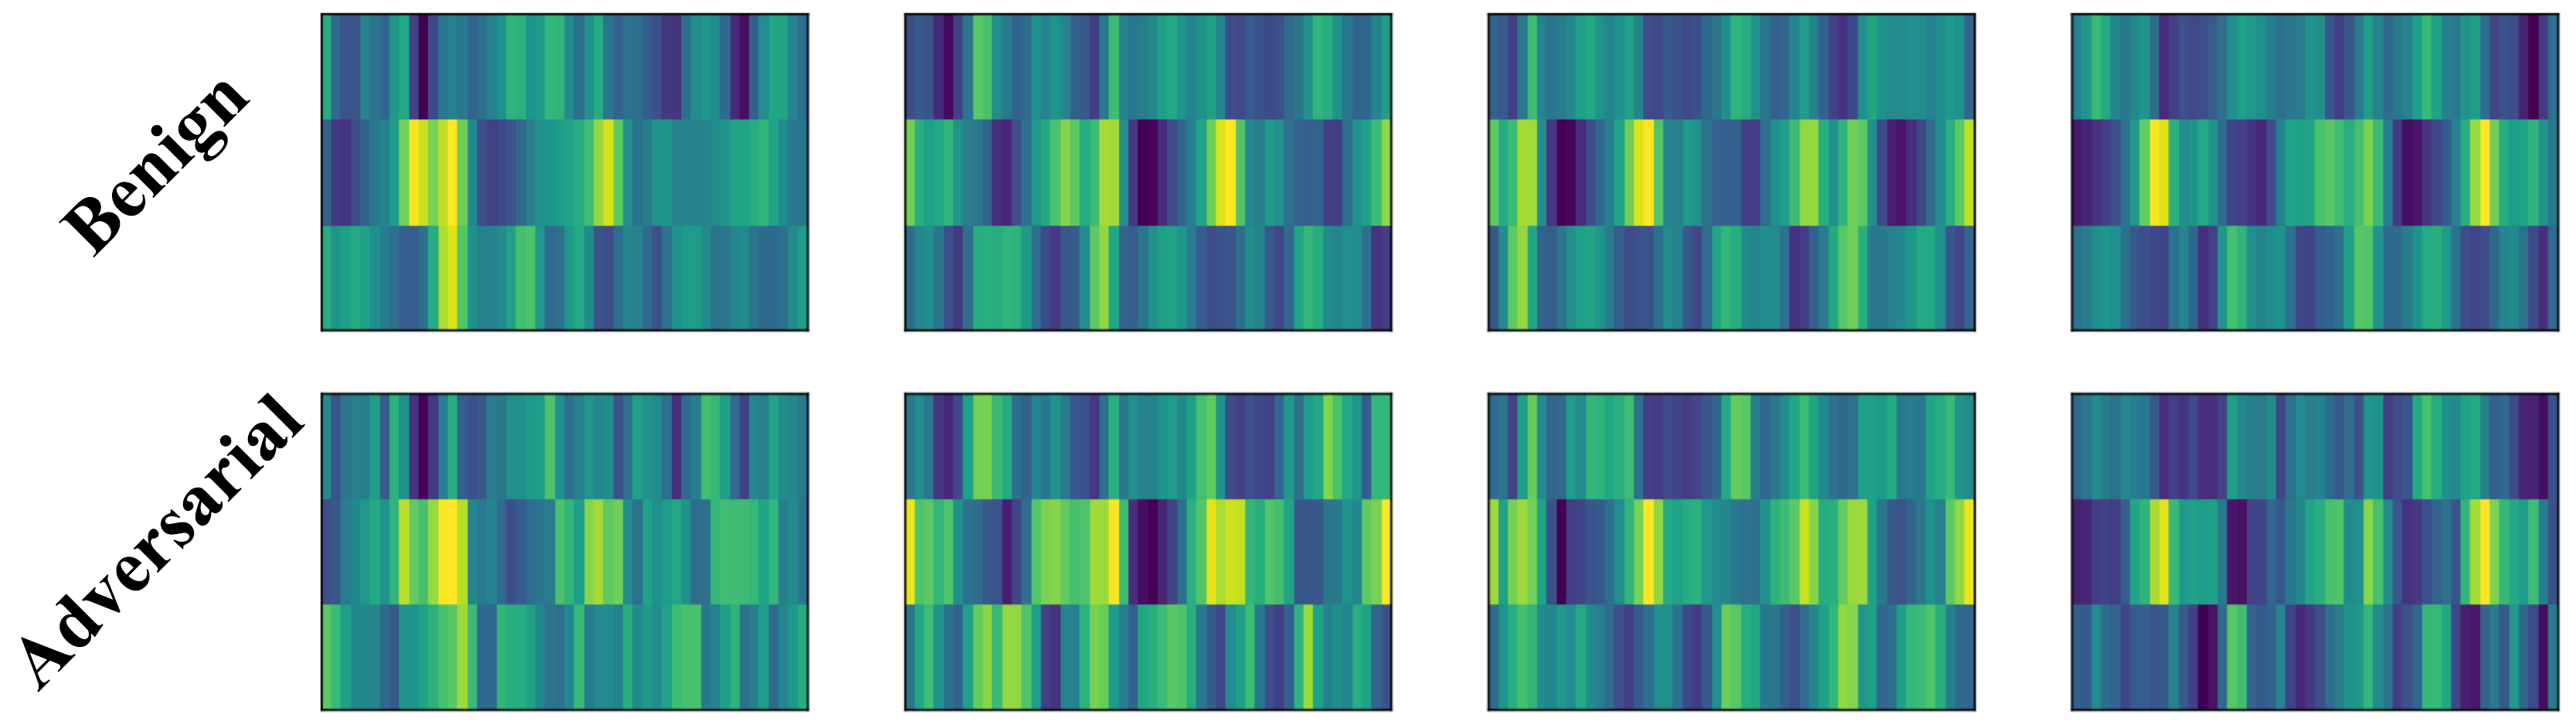}
  \caption{Adversarial examples of Predictive Attack on User. $\ell_\infty \; \epsilon = 0.3.$}
  \label{fig:adversarial_examples_user}
\end{figure}

\begin{figure*}
\centering
\includegraphics[width=0.60\linewidth]{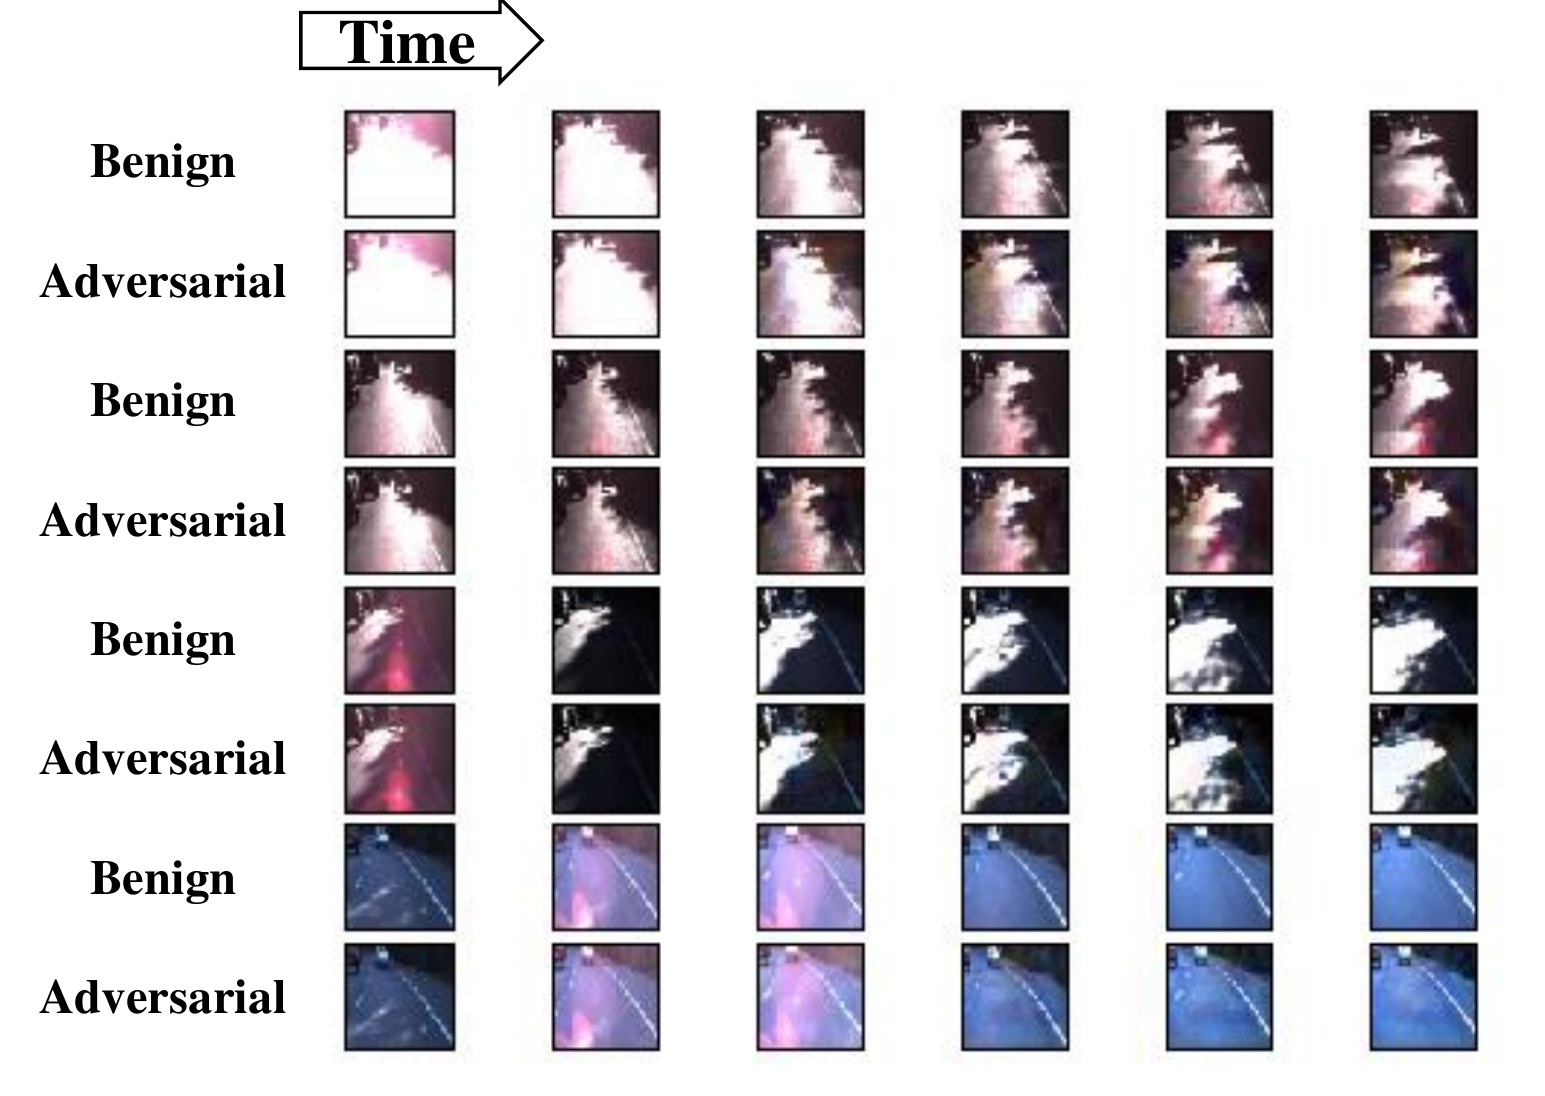}
  \caption{Adversarial examples of Predictive Attack on Udacity. $\ell_\infty \; \epsilon = 0.05.$}
  \label{fig:adversarial_examples_udacity}
\end{figure*}

\begin{figure}
\centering
\includegraphics[width=1.0\linewidth]{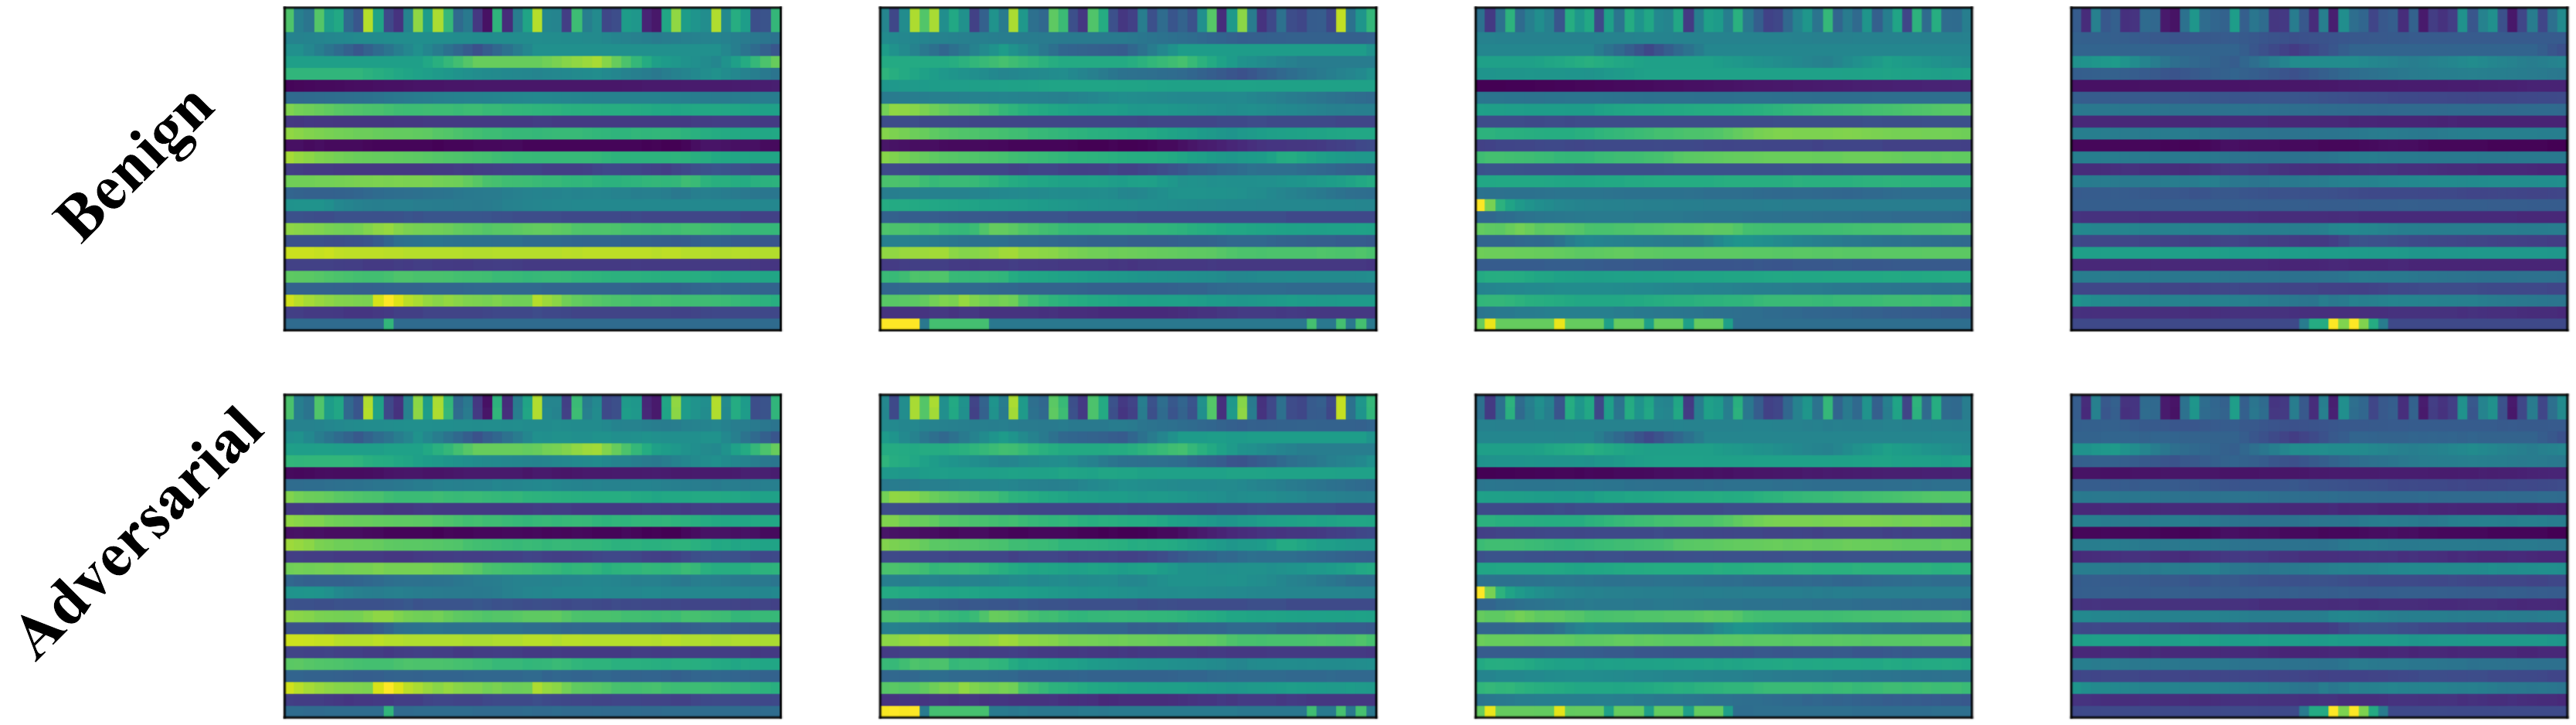}
  \caption{Adversarial examples of Predictive Attack on Energy. $\ell_\infty \; \epsilon = 0.02.$}
  \label{fig:adversarial_examples_energy}
\end{figure}

\section{Attack Performance with Different Targets}
\label{appendix:different-targets}
In order to evaluate the attack performance in more diverse targets, we increase the speed of target change. ``Target frequency'' refers to the speed at which the target changes. For example, the targets in \autoref{fig:target label} of the main paper correspond to frequency 2. By increasing the target frequency from 1 to 12, the results are summarized in \autoref{fig:multi-wave}. It is confirmed that Predictive Attack shows performance close to Clairvoyant Attack even when the target frequency is changed.

Overall, in the case of the classification task, the attack performances tend to decrease as the target frequency increases. We guess this is because the frequent target changes make the adversarial objective more difficult to achieve. On the other hand, Udacity and Energy, which are regression tasks, showed different results. We guess $y$ ranges of each training dataset affect the results. We assume it is easier to mislead a victim to yield an observed value in training than an unobserved value. As the target frequency increases too fast to follow, misleading a victim model to yield $y = 0$ would be advantageous as it can reduce the average TMSE. However, in the case of Energy, attacks would suffer from more difficulty since the zero is not observed in the $y$ range of the Energy training dataset. $y$ value of Energy is an energy consumption that has only positive values, while $y$ of Udacity is a steering angle, and it has positive and negative values crossing zero. 

\section{Variability of the Achieved Results.}
\begin{figure}
\centering
\includegraphics[width=0.95\linewidth]{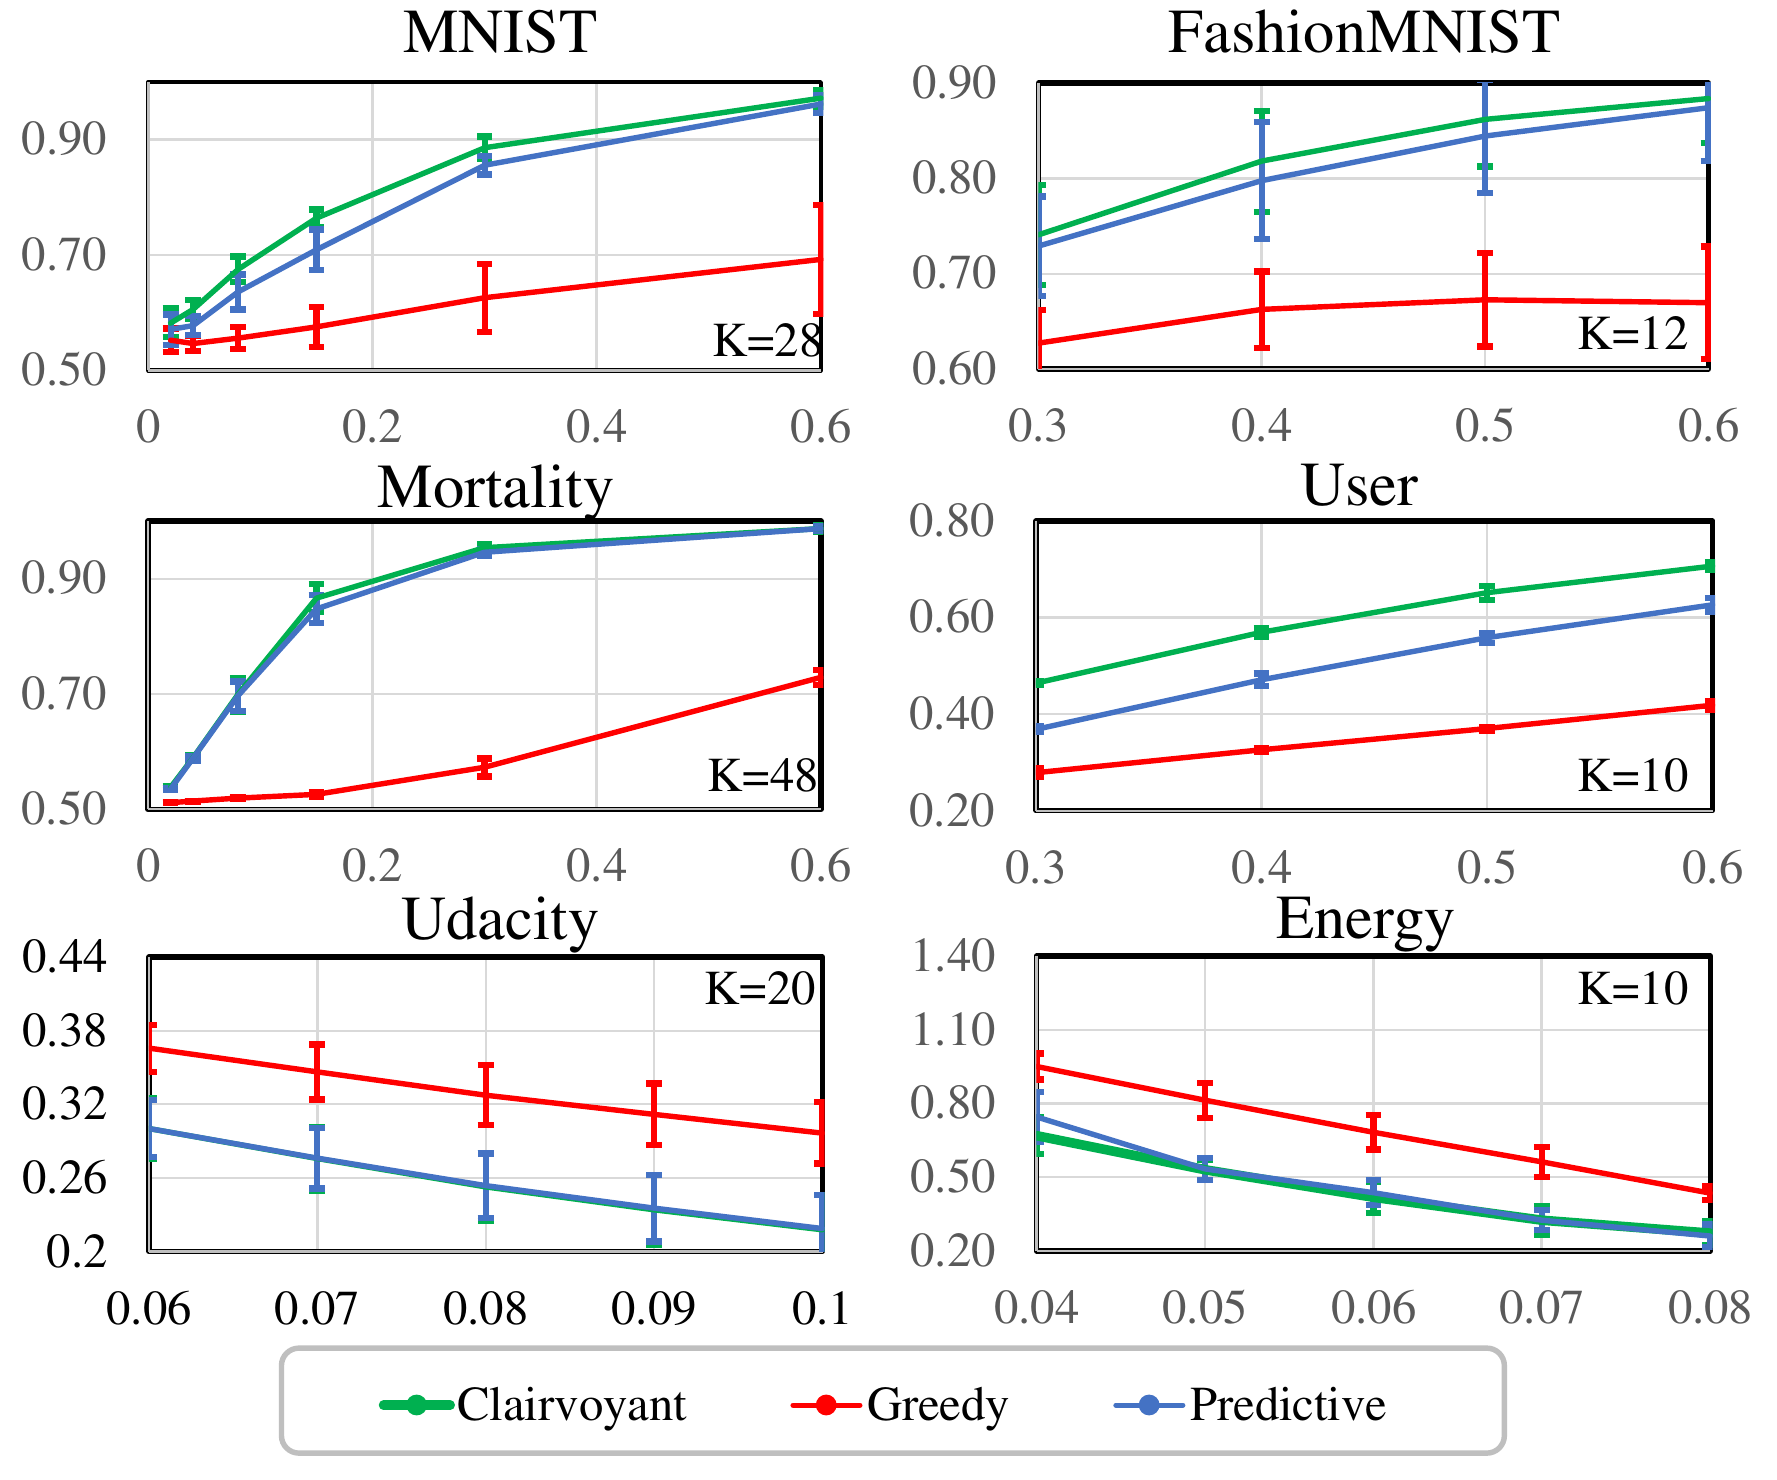}
%\vspace{-0.4em}
  \caption{Variability of the achieved results (Figure 5 in the main paper). We visualize 1$\sigma$ ranges of the results.}
  \label{fig:main-result-range}
%\vspace{-0.4em}
\end{figure}
\autoref{fig:main-result-range} is Figure 5 of the main paper with 1 sigma performance range ($-\sigma/\sqrt{n} \sim +\sigma/\sqrt{n}, n=3$). We exclude IID Attack to improve readability. We can check that Predictive Attack's performance ranges do not overlap with Greedy Attack's but overlap with Clairvoyant Attack's. It validates that Predictive Attack performs well in several trials consistently. Relatively, the ranges in FashionMNIST and Udacity are close compared with the other datasets. However, the actual performances of Greedy and Predictive are not close. In other words, the higher the performance of Greedy is, the higher the performance of Predictive is, and vice versa. To support that, we compute the performance correlations between Greedy and Predictive at the largest $\epsilon$, which are 0.99 and 0.75 in FashionMNIST and Udacity, respectively.

\section{Additional Transferability Test}
We evaluate the effectiveness of Predictive Attack in a black-box threat model, in addition to the gray-box assumption in the main paper. 
The attacker trains a surrogate model with a different architecture from the victim model and generates adversarial examples on the surrogate model. Then, the attacker applies the adversarial examples to a victim model.

We prepare two experiments regarding the structure of the surrogate model: 1) Different architecture in the number of the last linear layers, and 2) Different architecture in the dimension of LSTM's hidden state. We show the results on MNIST in Figure \ref{fig:transferability_test}. We measured relative attack performance compared to the white-box performance on the surrogate model. Predictive Attack is at least 45\% and 30\% effective for each case, even with the different architectures.
% We evaluate the effectiveness of Predictive Attack in a grey-box threat model, in addition to the white-box assumption. 
% %\JH{In this threat model, an attacker's strategy is transferability~\cite{delving}: adversarial examples generated on a model are occasionally effective to different models.} 
% In this threat model, an attacker uses transferability of adversarial examples~\cite{delving}: a fraction of adversarial examples generated on a model is effective to different models.
% The attacker trains a surrogate model and generates adversarial examples on the model. Then, the attacker applies the adversarial examples to a victim model.

% We prepare three experiments regarding the structure of the surrogate model: 1) Same structure as a victim model but trained with different parameter initializations, 2) Different structures in the number of the last linear layers, and 3) Different structures in the dimension of LSTM's hidden state. We show the results on MNIST in Figure \ref{fig:transferability_test}. We measured relative attack performance compared to the white-box performance on the surrogate model. If the victim model has the same structure as the surrogate model, Predictive Attack is 60.59\% effective. Also, Predictive Attack is at least 45\% and 30\% effective for the other cases, even with the different structures.

\begin{figure}
\centering
\includegraphics[width=1.0\linewidth]{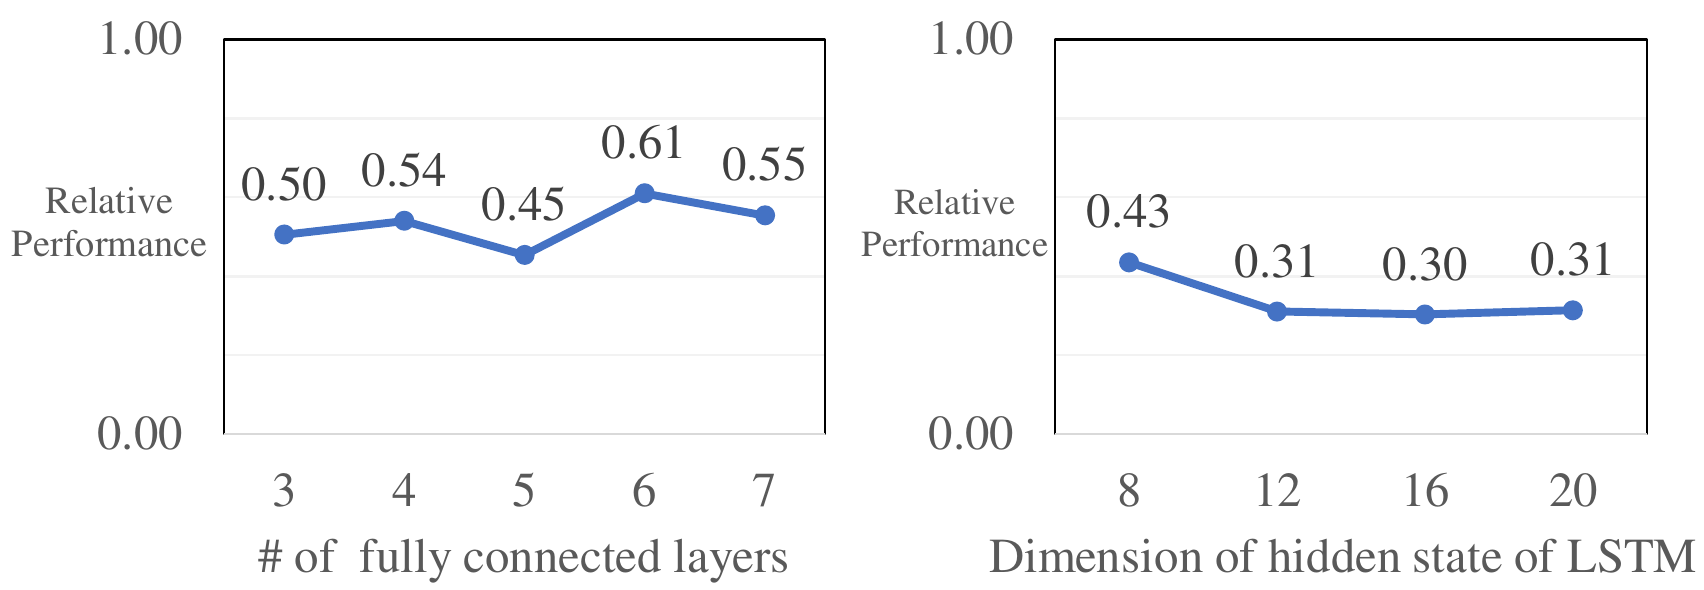}
  \caption{The relative performance of transferred adversarial examples compared to white-box attack fool rates on MNIST.
  Attacking a surrogate model with $\epsilon = 0.3$ constraints, Predictive Attack ($K=28$) generated the adversarial examples.
  Whitebox fool rate on the surrogate model is 0.98.
  We find Predictive Attack can achieve 30$\sim$61\% of white-box performance although the victim model has different architectures. Performances of five trials are averaged.}
  \label{fig:transferability_test}
\end{figure}

\section{Impact of the Number of Sequences in Monte-Carlo Computation}
\begin{figure}
\centering
\includegraphics[width=1.0\linewidth]{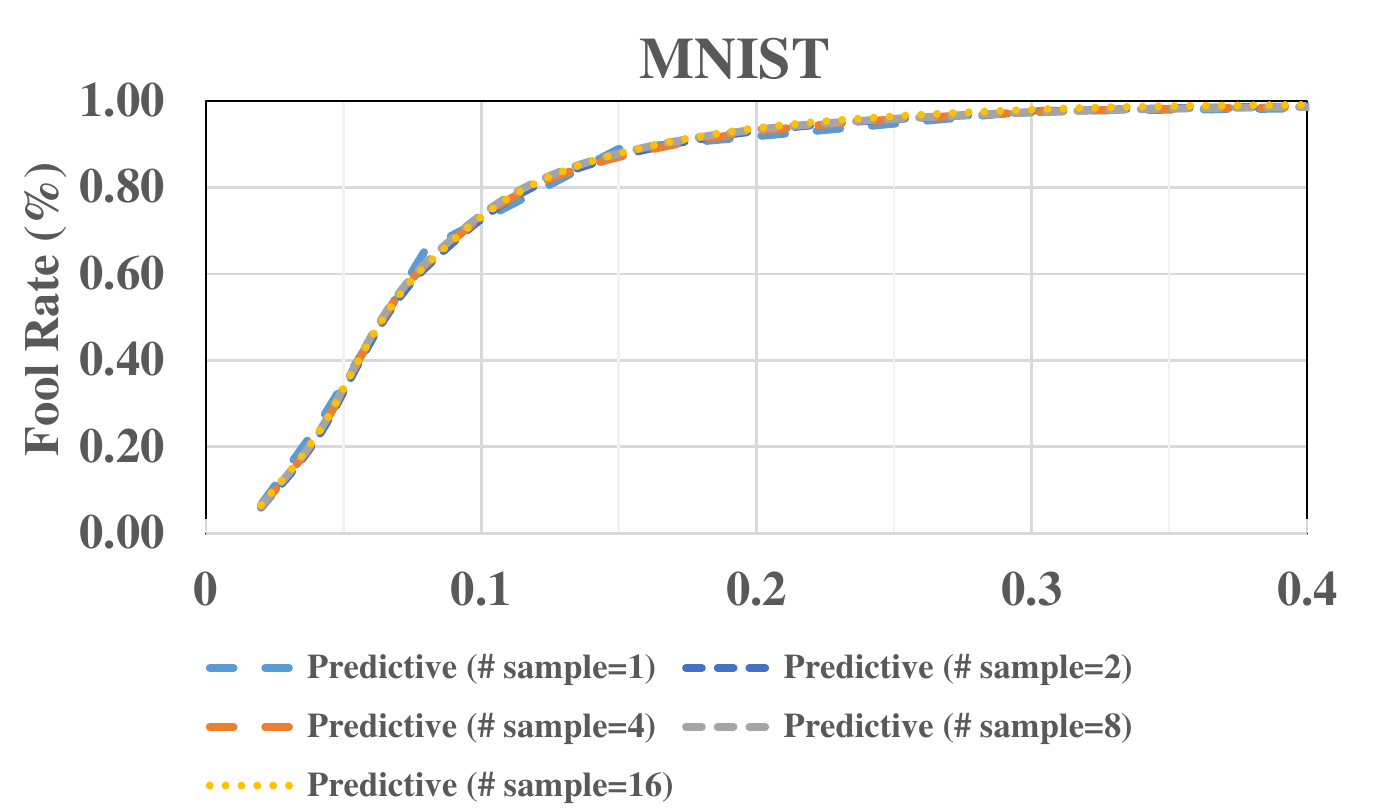}
  \caption{Impact of the number of sequences in Monte-Carlo simulation. Since there is no uncertainty in the dataset, so does its stochastic $Q_\phi$.
  Therefore, the performance does not depend on the number of samples.}
  \label{fig:num_of_monte_carlo}
\end{figure}
\begin{figure}
\centering
\includegraphics[width=1.0\linewidth]{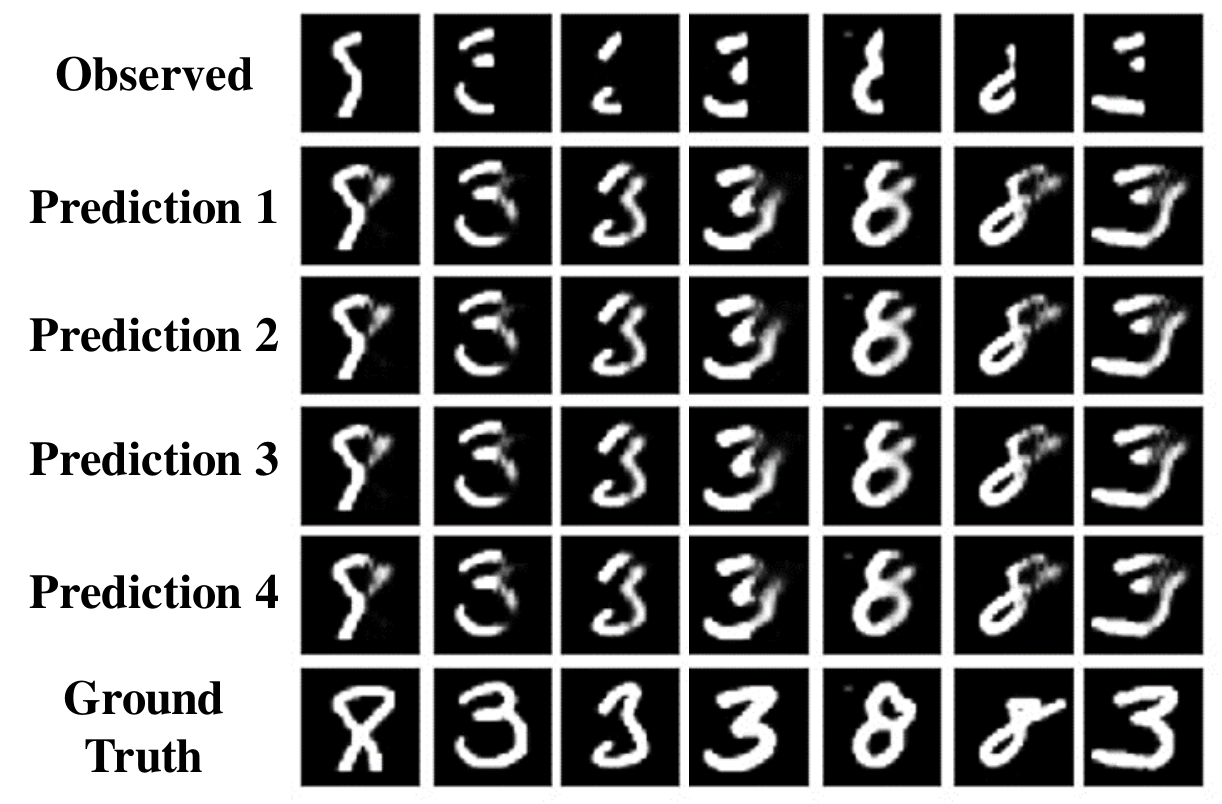}
  \caption{Prediction performance of a stochastic $Q_\phi$ on MNIST.
  We can see that multiple sampling produces similar digits.}
  \label{fig:mnist_stochastic_prediction_all}
\end{figure}

To fully demonstrate the correctness of our approach (\autoref{eq:predictive_attack_loss_full}) of Predictive Attack , we present attack performances with multi-samplings. We train new stochastic $Q_\phi$ that includes stochastic latent variables and, thus, produces different predictions for each sampling trial.\footnote{Chung , J. et al. 2015, ``A Recurrent Latent Variable Model for Sequential Data''}
Regardless of the number of sampling trials, the attack performances are very similar. We ascribe it to the task characteristic of MNIST that is almost deterministically predictable: the next column of a digit is almost identical to the current column.
%\JH{More MNIST samples?}
We show this characteristic in Figure \ref{fig:mnist_stochastic_prediction_all}. Multiple predictions of MNIST produce similar images.
%\section{G. Effect of Interval Differences}
% \section{G. Additional Related Work}
% \input{0_IJCAI22/background_relatedwork}
% \paragraph{Offline Evasion Attack.}
% After the first appearance of an adversarial attack~\cite{szegedy}, many attack variants emerged ~\cite{fgsm,pgd,fab}. Under an implicit assumption that an attacker can observe and perturb the entire inputs, they aim to improve attack performances with small perturbations. 
% We call them ``offline evasion attacks'' to clearly distinguish them from attacks of our interest. Due to the lack of online constraints, offline evasion attack is not practically applicable for online temporal models.
%  We propose a general formulation for online evasion attacks and study its practical impact on realistic scenarios.

\section{Impact of $\rm{MAX\_COUNT}$.}
\autoref{fig:iters} illustrates speed of convergence in terms of attack performances. x-axis is $\rm{MAX\_COUNT}$, and y-axis is attack performance. We can check the gradients of Predictive Attack's attack performances, which mean speed of convergence, are close to those of Clairvoyant Attack's.
\begin{figure}
\centering
\includegraphics[width=0.95\linewidth]{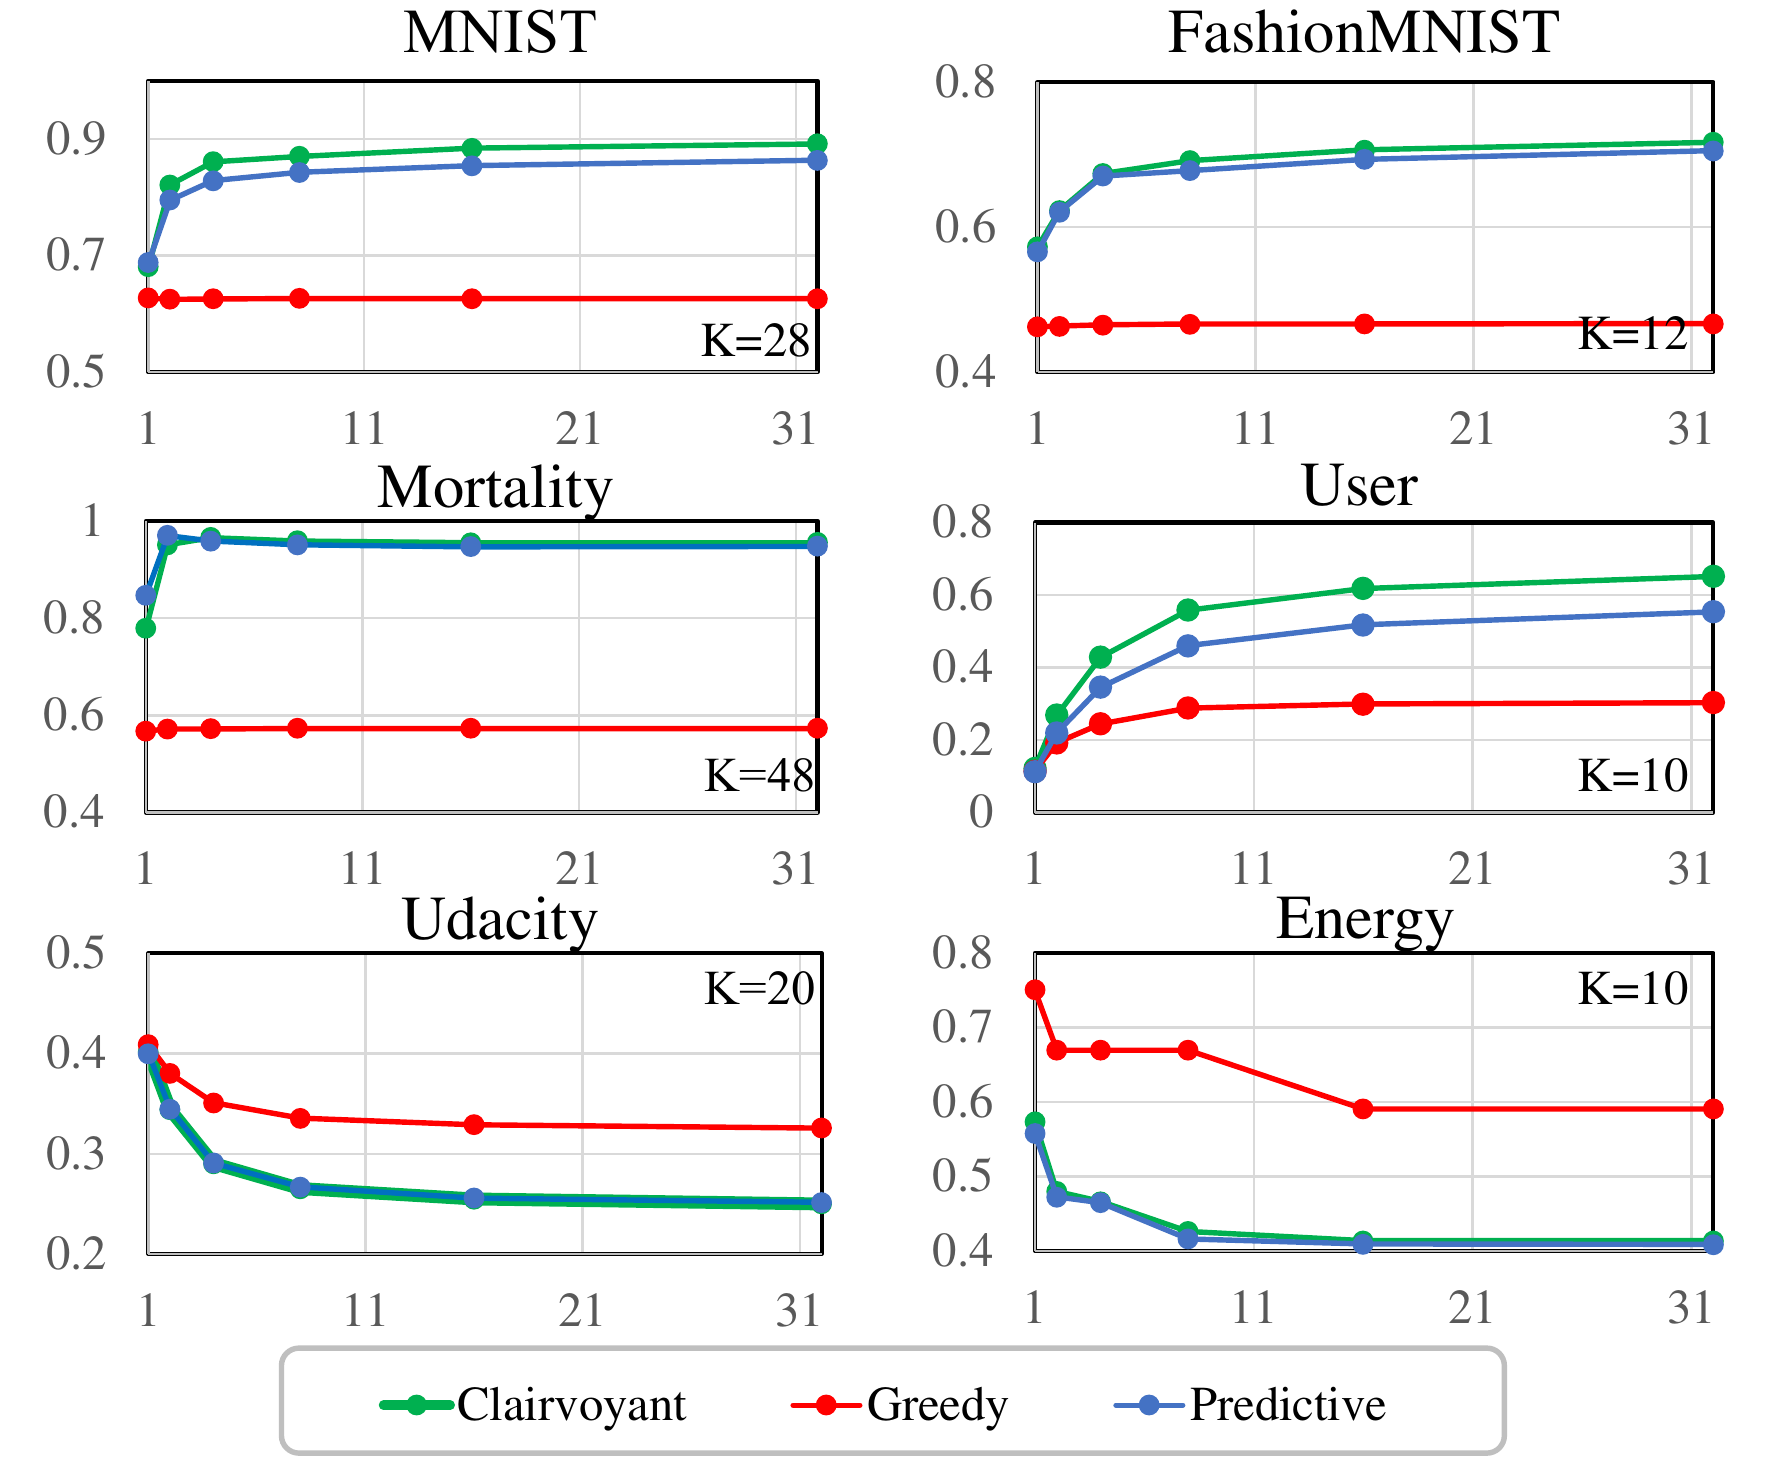}
%\vspace{-0.4em}
  \caption{Impact of $\rm{MAX\_COUNT}$. Predictive Attack's attack performances converge as fast as those of Clairvoyant Attack.}
  \label{fig:iters}
%\vspace{-0.4em}
\end{figure}

\section{Validation of Real-time Attack Implementation}
\label{appendix:real-time-attack-validation}
\begin{figure}[h]
\centering
\includegraphics[width=1.0\linewidth]{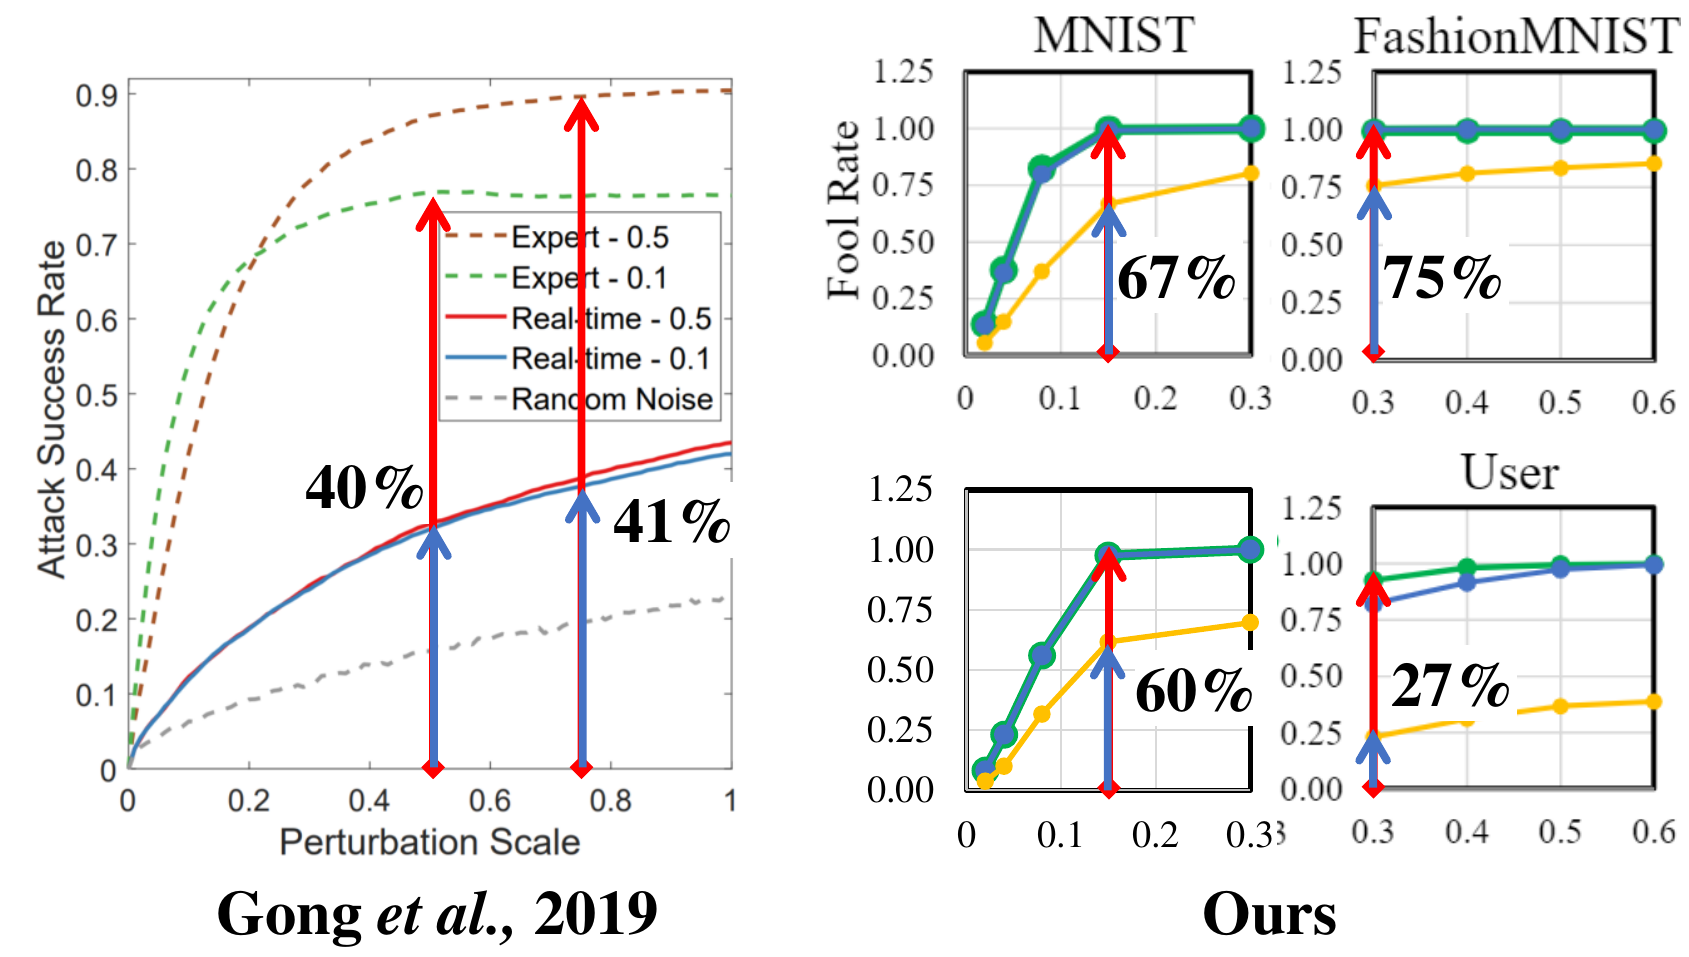}
  \caption{Implementation validation of the imitation learning-based real-time attack.  We demonstrate how the relative performances of imitation learning-based attacks to that of an expert are computed.
  Our implementation (right, yellow) achieves higher performances, compared to the original implementation (left, straight lines), because of the larger number of perturbation steps.}
  \label{fig:from_real_time_paper}
\end{figure}
We reimplement an imitation learning-based real-time attack~\cite{realtime_adversarial_attack} based on the public implementation\footnote{\url{https://github.com/YuanGongND/realtime-adversarial-attack}} because the original implementation has problem-specific constraints such as perturbation being restricted to five subsets of the entire time periods, while we consider the entire period for an attack. 
We replace the problem-specific expert \cite{differential_evolution} originally used for audio data with the general expert Clairvoyant ($K$=$L$).
To verify our implementation is correct, we measured the relative performance of the attack to an expert.
In particular, the performance is measured at $\epsilon$ where a performance of the expert converged (Figure \ref{fig:from_real_time_paper}).
The average relative performance of our implementation (right yellow, 57\%) is higher than that of the public implementation (left straight lines, 40$\sim$41\%). This difference comes from the number of time steps where perturbations are generated. While the original implementation allowed only five perturbation steps, our implementation generates perturbations for all time steps ($L$).
%\JH{A bit more details about how these numbers were measured?}

\section{Online Evasion Attack on Online Training}
It is meaningful to consider online training in an online evasion attack since it is frequently used to overcome the inefficiency of offline training in online tasks. Theoretically, we show online evasion attack on a victim changing with online training is the same as attacking a victim without online training. From a practical point of view, we also examine the challenge of attacking a recurrent model that changes its parameter.

Assuming the whitebox threat model as in the main paper, we assume that an attacker knows the parameter update rule $U(x_i, \theta_i): \mathbb{R}^n \times \mathbb{R}^N \rightarrow \mathbb{R}^N$ of the victim's online training where $N$ is the number of model parameters. In this setup, an online evasion attack can be similarly formulated by incorporating $U$ to the original problem. 
\begin{gather}
\boldsymbol{\delta}=\argmin_{\boldsymbol{\delta}=(\delta_1,\cdots,\delta_L) \in \Delta}\; 
\mathrm{Agg}
\left(\mathcal{L}^{\text{adv}}_1,\cdots,\mathcal{L}^{\text{adv}}_L\right),\;\mathrm{where} \label{eq:problem_definition_attack_loss_general}
\end{gather}
$\mathcal{L}^{\text{adv}}_i$ is the loss at time $i$: $\mathcal{L}^{\text{adv}}_i=\mathcal{L}(f(x_{i}+\delta_{i}, h^{\delta}_{i}, {\theta_i}), y^{a}_{i})$, and:
%$h^{\delta}_i$ is the hidden state of the RNN at time $i$:
\begin{gather}
h^{\delta}_i = g(x_{i-1}+\delta_{i-1},\;h^{\delta}_{i-1}), \label{eq:problem_definition_h_update} \\
\theta_{i} = U(x_{i-1}+\delta_{i-1},\;\theta_{i-1}).
\end{gather}
From this point of view, parameter $\theta_i$ can be considered as an additional hidden state.
If we denote ($h^{\delta}_i$,  $\theta_i$) with $h^{\delta'}_{i}$ and denote $g$ and $U$ as $g'$, 
we can rewrite the equation 2 and 3 as $
h^{\delta'}_i = g'(x_{i-1}+\delta_{i-1},\;h^{\delta'}_{i-1})
$.
It reduces to the original problem (Equation 1 $\sim$ 2 of the main paper). As long as we can predict future inputs, we can compute an exact model parameter $\theta_i$ as well as hidden state $h^{\delta}_i$; thus, we can conduct the proposed online evasion attack.

\section{Possible Defense}
We propose a simple idea of using adversarial training [M{\c{a}}dry \textit{et al}., 2018], which is an effective defense against offline evasion attacks, as a defense against online evasion attacks. Firstly, we assume that the length of the input (the number of time steps) is a constant $L$. Under this assumption, we can consider the $L$-step unfolded recurrent victim model as an offline model. Therefore, as with adversarial training on an offline model, we can perform adversarial training on the unfolded victim model against $L$-step adversarial examples, using a PGD attack that minimizes an adversarial loss at each time step.

However, this defense would not be effective against attacks over $L$-step. The reason is that the adversarial error on hidden states of a victim model accumulates as an attack continues. The attacker would eventually succeed in manipulating hidden states to produce wrong victim outputs. A victim might initialize a hidden state to a value (e.g., zero vector) to prevent the accumulation; however, it would degrade victim's clean task performance.
